# Supplementary material for: Light-induced cortical excitability reveals programmable shape dynamics in starfish oocytes
Source: arXiv:2409.08651 ancillary file (2024-09-13)
Supplement: Supplementary file 1 [file Supplementary_Information.pdf]

# Supplementary Information for "Light-induced cortical excitability reveals programmable shape dynamics in starfish oocytes"

**Jinghui Liu[1,2,*], Tom Burkart[3,*], Alexander Ziepke[3], John Reinhard[4,5], Yu-Chen Chao[1,6], Tzer Han Tan[1,7], S. Zachary Swartz[8,9], Erwin Frey[3,10,†], Nikta Fakhri[1,†]**

This Supplementary Information includes: Supplementary Notes 1-5, Supplementary Movies 1-11, Supplementary Tables 1-5, and Supplementary Figures 1-7.

**List of supplementary tables**

S1 Reaction-diffusion parameters for native GEF, Ect2 . . . 7
S2 Reaction-diffusion parameters for Opto-GEF . . . 8
S3 Parameters for modeling varied light illumination . . . 9
S4 Parameters for modeling Rho dynamics . . . 10
S5 Parameters for modeling shape dynamics . . . 12

**List of supplementary figures**

S1 "Dose-dependent" phenotypes of Opto-X oocytes under photoactivation . . . 4
S2 Optogenetic responses for "dose-imbalanced" Opto-X oocytes. . . . 5
S3 Membrane-plane photoactivation and Opto-GEF* recruitment. . . . 6
S4 Transition between localized and propagating excitations. . . . 10
S5 Phase portrait analysis and excitation threshold . . . 13
S6 Transitions from localized Rho responses to propagating excitations . . . 17
S7 Extraction of oocyte shape from time series data . . . 20

**1 Supplementary notes** **3**
1 Experimental implementation of Opto-X assays in starfish oocytes . . . 3
2 Modeling . . . 3
2.1 Simulations of the chemical module . . . 3
2.2 Simulations of the mechanical module . . . 11
3 Excitation threshold and activation . . . 12
3.1 Excitation threshold . . . 12
3.2 State perturbations and threshold perturbations. . . . 14
4 Experimental and modelling verification of proposed interactions . . . 15
4.1 Rho . . . 15
4.2 Myosin . . . 15
4.3 Opto-Null . . . 16
4.4 Opto-GEF* . . . 16
5 Classification of contraction phenotypes . . . 19

---

[1]Department of Physics, Massachusetts Institute of Technology, Cambridge, MA, USA. [2]Center for Systems Biology Dresden, Dresden, Germany. [3]Arnold Sommerfeld Center for Theoretical Physics and Center for NanoScience, Department of Physics, Ludwig Maximilian University of Munich, Munich, Germany. [4]Medical Biochemistry and Molecular Biology, Saarland University, Homburg, Germany. [5]Physiology Course, Marine Biological Laboratory, Woods Hole, MA, USA. [6]School of Engineering and Applied Sciences, Harvard University, Cambridge, MA, USA. [7]Current address: Department of Physics, University of California San Diego, La Jolla, CA, USA. [8]Whitehead Institute for Biomedical Research, Cambridge, MA, USA. [9]Eugene Bell Center for Regenerative Biology and Tissue Engineering, Marine Biological Laboratory, Woods Hole, MA, USA. [10]Max Planck School Matter to Life, Munich, Germany. [*]These authors contributed equally: Jinghui Liu, Tom Burkart. [†]Corresponding authors: frey@lmu.de, fakhri@mit.edu.

**2 Movie captions** **21**
S1 Reversible oocyte deformations driven by patterned illumination with Opto-GEF assay. . . . . . . . . . . . 21
S2 Mid-plane view of membrane Rho-GTP dynamics driven by continuous global illumination. . . . . . . . . 21
S3 Near-membrane view of membrane Rho-GTP dynamics driven by continuous global illumination. . . . . . 21
S4 Simulation of a self-sustained traveling Rho wave following local activation. . . . . . . . . . . . . . . . . . . 21
S5 Reversible oocyte deformations driven by patterned illumination expressing Opto-GEF* assay. . . . . . . . 21
S6 Opto-GEF* assay-expressing oocytes exhibit pinching or unguided SCW upon local activation. . . . . . . . 21
S7 Wild-type oocyte exhibits guided SCW under hormone induction. . . . . . . . . . . . . . . . . . . . . . . . 21
S8 Opto-GEF assay-expressing oocyte exhibits guided SCW under continued global activation. . . . . . . . . . 21
S9 Irreversible Opto-GEF assay-expressing oocyte lysis driven by global illumination. . . . . . . . . . . . . . . 21
S10 Irreversible Opto-GEF* assay-expressing oocyte lysis driven by global illumination. . . . . . . . . . . . . . 21
S11 Extreme irreversible Opto-GEF assay-expressing oocyte lysis driven by global illumination. . . . . . . . . 21

**3 References** **22**

## Supplementary notes

### 1 Experimental implementation of Opto-X assays in starfish oocytes

Experimentally, we surveyed the deformation phenotypes by tuning (i) types of optically-recruited GEF variants, and (ii) illumination parameters from the optical manipulation. In practice, by microinjecting mixtures of mRNAs into prophase-arrested starfish oocytes and waiting for overnight expression, we naturally generate a spectrum of oocytes that carry more factors of variability, such as doses and ratios of proteins in the Opto-X assay, even when the same mixture was prepared and injected. The interpretation of our experimental results was made based on a consistent understanding of all variability factors. In the following, we discuss in detail the spectrum of our observations and the link to features of the optogenetic system.

The first factor that significantly impacted the type of optogenetic responses an oocyte exhibits is the expression level of Opto-X assay proteins before photo-manipulation onsets (Fig. S1a). For Opto-GEF* assay, oocytes with visibly higher Cry2PHR cytosolic signals have higher probability to show a moving contraction front ("decaying SCWs") instead of a stationary one ("pinches"), when placed under the same regional illumination (Fig. S1b). For Opto-GEF assay, global illumination with the same light condition generates a spectrum of oocyte responses. While all oocytes show the relocation of cytosolic Cry2PHR signal onto membrane upon activation, fast guided SCWs and subsequent lysis were only observed in the fraction of oocytes with a high initial Cry2PHR cytosolic signal (corresponding to a high density of photo-sensitive domains in cytosol) and a sufficient build-up rate of membrane Cry2PHR (corresponding to the cross-product of photo-sensitive domain and membrane anchor domain densities, Fig. S1c). Consistent with the dose-dependent observation, the activation time it takes for Opto-GEF oocytes to kick start the fast guided SCWs are also vastly different (20 min – 1 hr). This observation motivated us to extend the experimental routine, such that after batch injection a screening was made to select oocytes with the highest fluorescence density of Cry2PHR to bring into illumination experiments. Since the CIBN membrane anchor is fluorescently-tagged in the same excitation channel as the photoactivation, we recorded the CIBN membrane anchor distribution only after the illumination was completed. The Cry2PHR and CIBN profile then permits us to crosscheck the effective strengths from first-order domain-domain binding and the observed oocyte responses.

We prepared the mRNA mixture for batch injection of the Opto-X assays to have comparable stoichiometry between Cry2PHR and CIBN components, in order to have an optimized recruitment rate. However, we note that for Opto-GEF* assay, the high-dose expression of exogenous GEF in a prophase-arrested oocyte can lead to misshapes and spontaneous lysis in the absence of optogenetic effects (Fig. S2a). Therefore for the expression of Opto-GEF* assay, we identified the proper injection concentration by preparing a ladder of undiluted CIBN mRNA mixed with different folds of dilution in the Cry2PHR mRNAs. Only oocytes from the proper dilution folds of Cry2PHR mRNA where no batch misshapes can be observed were used for photoactivation purposes. We discarded any oocytes that showed illumination-nonspecific contractile responses (<10%) using the expected correlation between Opto-GEF* accumulation and oocyte shape deformation as a readout.

The imbalance of stoichiometry between Cry2PHR and CIBN that were set up in the Opto-GEF* assay – higher expression levels of CIBN domains – did not bring out any notable side effects in our experiments, when compared to the balanced scenario. However, we note that the reversed stoichiometry order, where the Cry2PHR domains are significantly more concentrated, should be avoided. In the rare cases of Opto-GEF* assay expression where the CIBN domains are of very low presence compared to Cry2PHR (despite the stoichiometry set up in the mRNA mixture), a light-dependent clustering of Cry2PHR proteins in the oocyte cytosol was observed (Fig. S2b). This is likely associated with the Cry2-based homo-oligomerization reactions that have been reported and utilized in other works[1]. Indeed, when we expressed high levels of only the Cry2PHR protein in oocytes, similar clusters in cytosol were observed (Fig. S2c). We similarly ruled out results from these oocytes (<5%). We conclude from these observations that dose and stoichiometry controls for proteins in living cells are important for interpreting factors of variability in optogenetic experiments.

Finally, we note that all optogenetic experiments we presented in main text were performed with point-scanning illumination focused on the medium z-plane of the oocyte. This choice of activation and imaging comes from our need to acutely observe shape deformation and boundary recruitment. However, it is possible to use the same optogenetic assays to perform activation on a membrane plane (Fig. S3). How to resolve fine control of membrane activation pattern using a cytosolic photosensitive domain (Cry2PHR) would then be of interest for more sophisticated photomanipulation purposes.

### 2 Modeling

In the following, we present the details of the numerical methods used to simulate the chemomechanical dynamics in starfish oocytes in wild-type situations as well as for optogenetically treated oocytes. The simulations are split into a chemical module and a mechanical module (Fig. 2).

#### Simulations of the chemical module

The chemical module contains the reaction-diffusion dynamics of all involved proteins in a fixed geometry. More precisely, this includes the native GEF Ect2, the optogenetic GEF, and the Rho proteins. The reaction-diffusion dynamics were solved

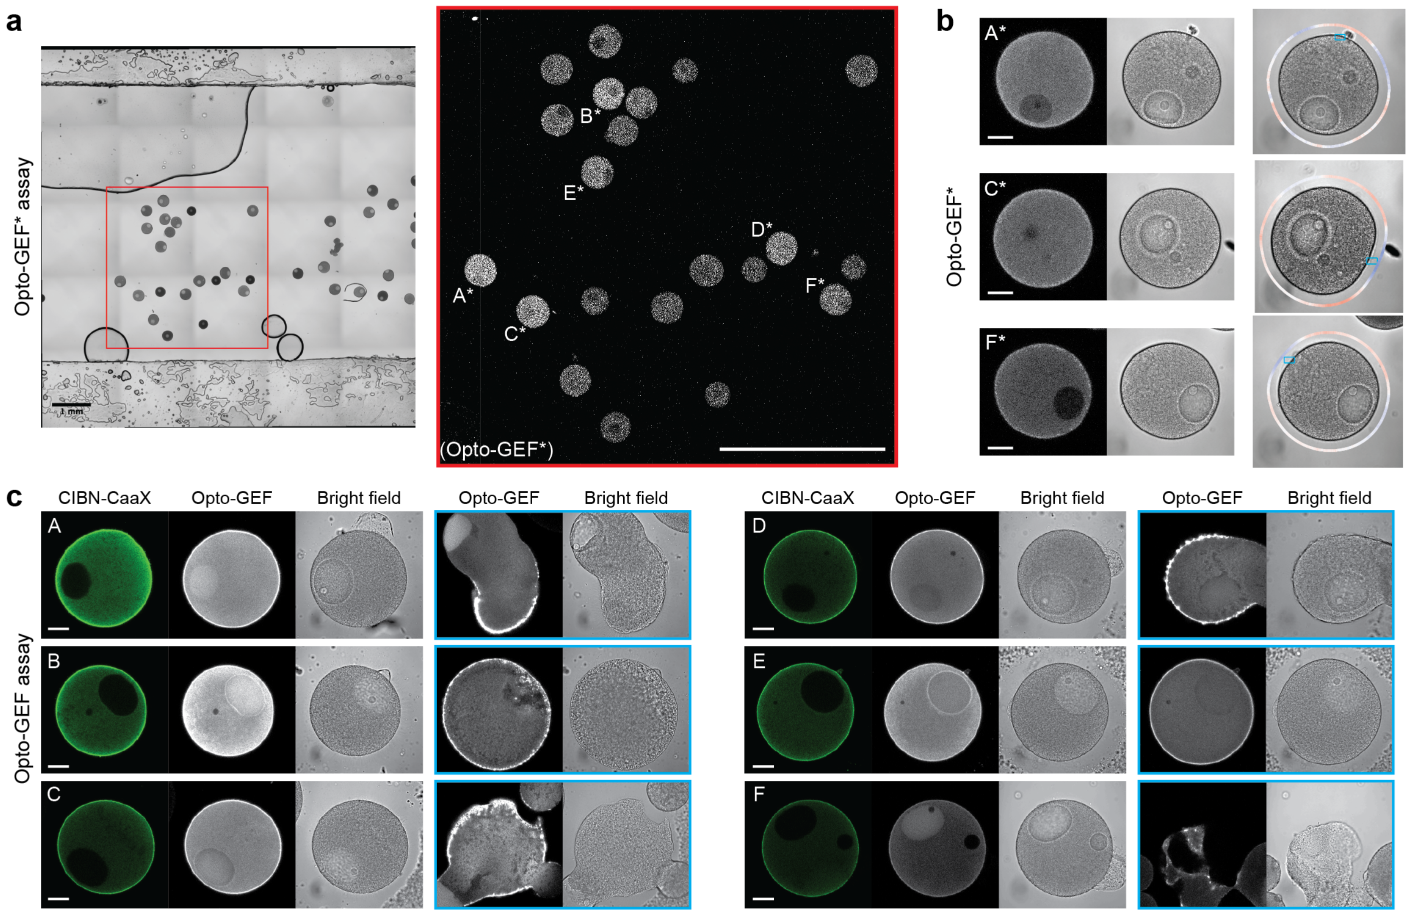


**Supplementary Fig. S1 | Opto-X oocytes exhibit varying chemomechanical responses that are "dose-dependent" upon photoactivation. a,** Fluorescence (left) and bright field (right) snapshot of a collection of oocytes expressing Opto-GEF* assay. The snapshot was taken before onset of regional illumination. Scale bar: 50 $\mu$m. **b,** Quantification of Opto-GEF* expression levels per oocyte for the collection shown in **a**. Oocytes (i)-(iii) labelled in **a** and **b** exhibited respectively weak pinching, strong pinching and decaying surface contraction wave (SCW) behaviors upon onset of the same intensity and frequency of regional illumination (same as in Extended Data Fig. 8a, c). **c,** CIBN-eGFP (left) and Opto-GEF (right) fluorescence channel snapshot of a collection of oocytes expressing Opto-GEF assay. The snapshot was taken at the onset of global illumination. Scale bar: 50 $\mu$m. **d,** CIBN-eGFP (left) and Opto-GEF (right) fluorescence channel snapshot of the collection of oocytes shown in **c**. The snapshot was taken at the end of global illumination. Oocytes (i)-(iii) labelled in **c** and **d** exhibited cell lysis at the end of illumination while the others underwent rounding and stiffening driven by accumulating membrane Opto-GEF but no lysis over an illumination of up to 2 h. Scale bar: 50 $\mu$m.

in finite element simulations using COMSOL Multiphysics 6.0. In accordance with typical experimental datasets and to improve simulation speed, we chose to simulate a slice of the oocyte as a representation of the full (three-dimensional) oocyte. Previous work showed that this dimensional reduction captures all relevant dynamics, and an extension to three dimensions is possible yet cumbersome[2]. In the following, all bulk concentrations are therefore stated as per-area concentrations (instead of per-volume), and similarly concentrations on the membrane are taken to be per-length (instead of per-area), with all reaction rates adapted accordingly. Note that the reaction-diffusion dynamics explicitly account for the de-/attachment of particles from/to the membrane, which is typically denoted in terms of a reactive boundary condition[3]:

$$D_{\mathrm{J}}\, \hat{\mathbf{n}}_{\mathcal{S}} \cdot \nabla u_{\mathrm{J}}|_{\mathcal{S}} = f\left(\{u_{\mathrm{j}}\}, \{u_{\mathrm{J}}|_{\mathcal{S}}\}\right) . \tag{1}$$

In general, we use uppercase subscripts $(\cdot)_J$ to indicate cytosolic concentrations and lowercase subscripts $(\cdot)_j$ for membrane concentrations. The membrane object is denoted by $\mathcal{S}$, where subscripts ($(\cdot)_{\mathcal{S}}$ and $(\cdot)|_{\mathcal{S}}$) indicate that a quantity is to be evaluated on the membrane. In particular, the vector $\hat{\mathbf{n}}_{\mathcal{S}}$ is the normal vector on the membrane. At the boundary, diffusive fluxes onto/from the membrane $D_J\, \hat{\mathbf{n}}_{\mathcal{S}} \cdot \nabla u_{\mathrm{J}}|_{\mathcal{S}}$ are balanced by reactive fluxes on the membrane $f\left(\{u_{\mathrm{j}}\}, \{u_{\mathrm{J}}|_{\mathcal{S}}\}\right)$. Below, we state the reaction-diffusion equations for all involved components, as well as the corresponding parameter choices.

*Native Ect2.* The dynamics of the native Ect2 have been analyzed previously in the context of wild-type surface contraction waves[2]. There, it was proposed that Ect2 can be phosphorylated by the kinase-active Cdk1-cyclinB complex (Cdk1). Only

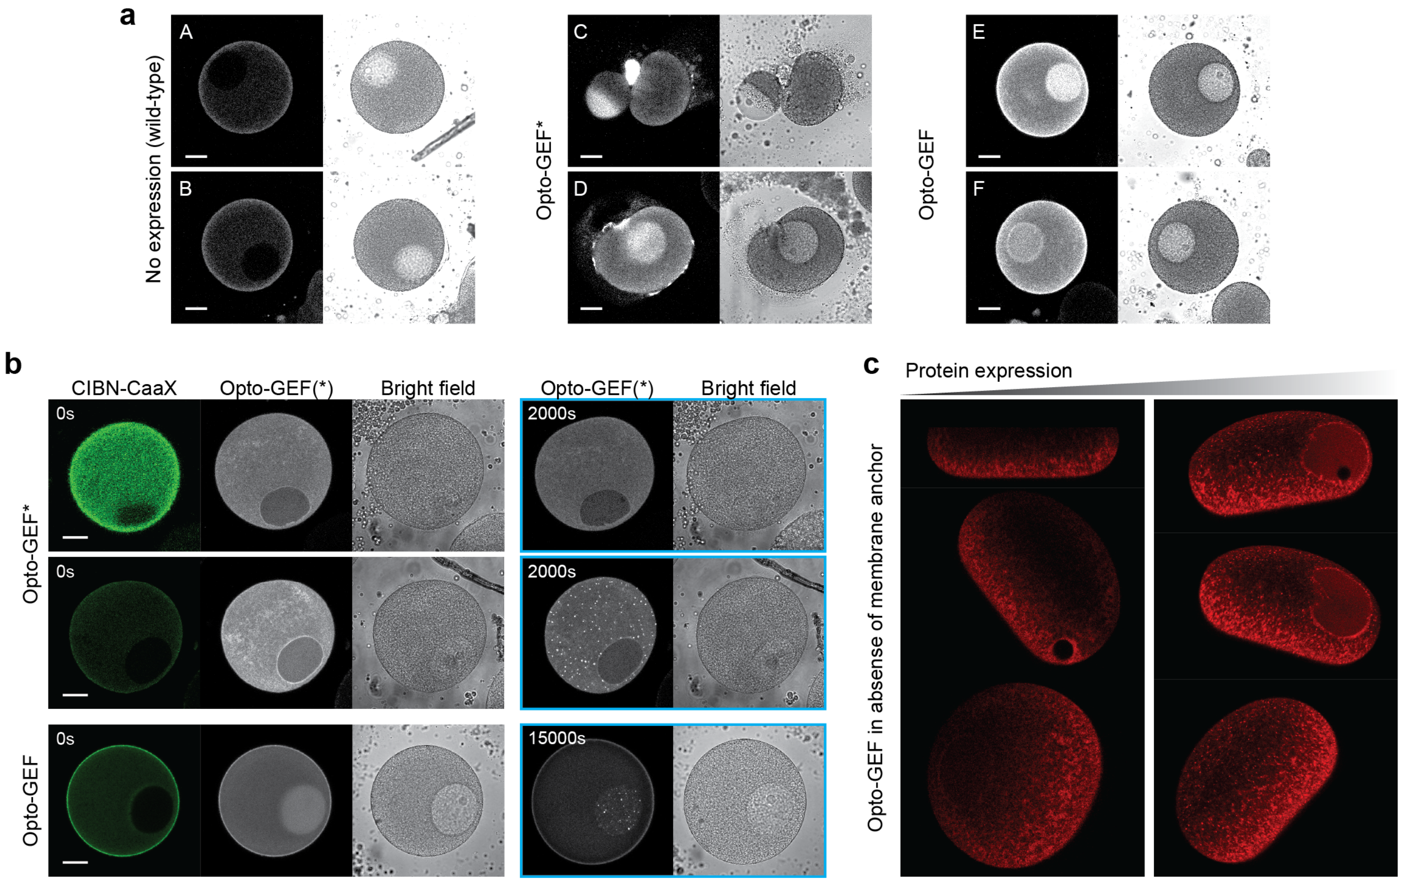


**Supplementary Fig. S2 | Optogenetic responses for GEF*-overdosed and Cry2PHR-CIBN stoichiometry-imbalanced Opto-X oocytes.** **a,** Cry2PHR fluorescence (left) and bright-field snapshots of oocytes expressing high levels of (i) Opto-GEF, (ii) Opto-GEF* assays and as compared to (iii) empty oocytes. The snapshots were taken 18 h after the microinjection of each type of assay mRNAs into the same batch of extracted oocytes. Scale bar: 50 $\mu$m. **b,** Time-lapse multi-channel snapshots of a representative oocyte where the expression of Opto-GEF and Opto-GEF* assay is dominated by the Cry2PHR protein but not the CIBN membrane anchor. Each oocyte was placed under continuous global illumination at 0.1 Hz that lasted for 30 min to 4 h. Scale bar: 50 $\mu$m. **c,** Fluorescence snapshot of a representative oocyte expressing high levels of Cry2PHR protein alone. The 3D view was reconstructed using z-stack slices that are $0.25 \mu m$ apart each. Scale bar: 50 $\mu$m.

the unphosphorylated proteins are considered to catalyze the nucleotide exchange of Rho, and only those are assumed to be membrane-binding[4]. Therefore, we distinguish between phosphorylated and unphosphorylated Ect2 proteins only in the cytosol ($u_{\mathrm{Ep}}$ and $u_{\mathrm{E}}$, respectively), whereas membrane-bound proteins are always unphosphorylated ($u_{\mathrm{e}}$). The generic reaction-diffusion equations for these proteins are

$$\partial_t u_{\mathrm{Ep}} = D_{\mathrm{E}} \nabla^2 u_{\mathrm{Ep}} + f_{\mathrm{Ep}}(u_{\mathrm{Ep}}, u_{\mathrm{E}}), \tag{2}$$
$$\partial_t u_{\mathrm{E}} = D_{\mathrm{E}} \nabla^2 u_{\mathrm{E}} + f_{\mathrm{E}}(u_{\mathrm{Ep}}, u_{\mathrm{E}}), \tag{3}$$
$$\partial_t u_{\mathrm{e}} = D_{\mathrm{e}} \nabla_{\mathcal{S}}^2 u_{\mathrm{e}} + f_{\mathrm{e}}\big(u_{\mathrm{Ep}}|_{\mathcal{S}}, u_{\mathrm{E}}|_{\mathcal{S}}, u_{\mathrm{e}}\big). \tag{4}$$

Here, the first term in each partial differential equation (PDE) denotes diffusion. Note that the diffusion constants in the cytosol and on the membrane ($D_{\mathrm{E}}$ and $D_{\mathrm{e}}$; values for parameters listed in Table S1), as well as the diffusion operators (Laplace operator $\nabla^2$ and Laplace-Beltrami operator $\nabla_{\mathcal{S}}^2$), differ from each other.

The second term in the PDEs accounts for mass-conserving reactions of the various Ect2 conformations. Cdk1, which was identified to effectively inhibit the enzymatic activity of Ect2[4], mediates the phosphorylation of Ect2 at a concentration-dependent rate $k_{\mathrm{Cdk1}}$ following Michaelis-Menten kinetics[2]. The Michaelis-Menten constant is $K_{\mathrm{p}}$. Dephosphorylation is assumed to happen at a constant rate $k_{\mathrm{dP}}$ as well as autocatalytically at a feedback rate $k_{\mathrm{fb}}$.

In addition, bulk-boundary coupling is accounted for by linear binding and unbinding of unphosphorylated Ect2 to and

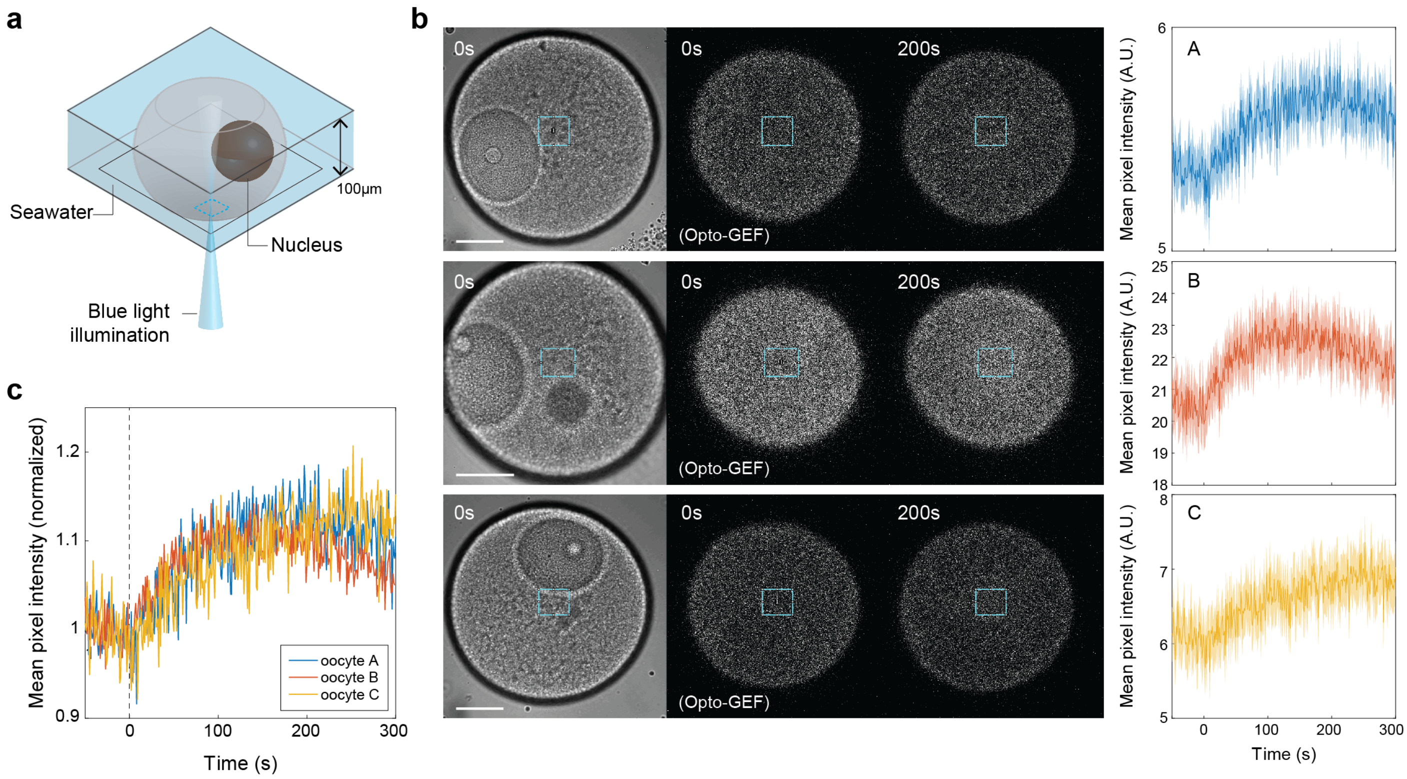


**Supplementary Fig. S3 | Regional illumination at the membrane plane induces chemomechanical responses on comparable timescales compared to nucleus-plane illumination. a,** Time-lapse multi-channel snapshots of 3 representative oocytes expressing Opto-GEF* assay and placed under membrane-plane regional illumination. Cyan boxes show the outline of illumination sites. The regional illumination (1 Hz) was made on the same single z-plane as the imaging and lasted for 200 s. Scale bar: 50 $\mu$m. **b,** Quantification of Cry2PHR intensity kinetics as a function of time for the illumination experiments shown in **a**.

from the membrane at rates $k_{\text{on/off,e}}$. In total, the used reaction terms read

$$f_{\text{Ep}}(u_{\text{Ep}}, u_{\text{E}}) = \frac{k_{\text{Cdk1}}\, u_{\text{E}}}{K_{\text{p}} + u_{\text{E}}} - (k_{\text{dP}} + k_{\text{fb}} u_{\text{E}}) \cdot u_{\text{Ep}}\,, \tag{5}$$

$$f_{\text{E}}(u_{\text{Ep}}, u_{\text{E}}) = -\frac{k_{\text{Cdk1}}\, u_{\text{E}}}{K_{\text{p}} + u_{\text{E}}} + (k_{\text{dP}} + k_{\text{fb}} u_{\text{E}}) \cdot u_{\text{Ep}}\,, \tag{6}$$

$$f_{\text{e}}\big(u_{\text{Ep}}|_{\mathcal{S}}, u_{\text{E}}|_{\mathcal{S}}, u_{\text{e}}\big) = k_{\text{on,e}}\, u_{\text{E}}|_{\mathcal{S}} - k_{\text{off,E}}\, u_{\text{e}}\,. \tag{7}$$

Since phosphorylated Ect2 is assumed to have no membrane binding, we use no-flux boundary conditions for this conformation. For unphosphorylated Ect2, the reactive boundary conditions correspond to the reactions of membrane-bound Ect2, resulting in the following set of boundary conditions:

$$\hat{\mathbf{n}}_{\mathcal{S}} \cdot \nabla u_{\text{Ep}}|_{\mathcal{S}} = 0\,, \tag{8}$$

$$D_{\text{E}}\, \hat{\mathbf{n}}_{\mathcal{S}} \cdot \nabla u_{\text{E}}|_{\mathcal{S}} = -k_{\text{on,e}}\, u_{\text{E}}|_{\mathcal{S}} + k_{\text{off,E}}\, u_{\text{e}}\,, \tag{9}$$

In the numerical simulations, the Cdk1 dynamics are not modeled explicitly, and instead we prescribe a decaying spatial gradient to represent the wild-type guiding mechanism:

$$k_{\text{Cdk1}}(\mathbf{x}, t) = \big(k_{\text{Cdk1,0}} - \alpha_{\text{Cdk1}}\,(x - R)\big) \cdot \left(1 - \frac{t}{\tau_{\text{Cdk1}} + t}\right)\,. \tag{10}$$

Here, $k_{\text{Cdk1,0}}$ corresponds to the Cdk1 concentration after nuclear envelope breakdown at the vegetal pole (VP), $\alpha_{\text{Cdk1}}$ is the slope of the gradient, and $\tau_{\text{Cdk1}}$ is the characteristic time scale at which the gradient decays. Note that neither the exact shape of the gradient nor the type of temporal decay is decisive for the observed dynamics, due to the generic bistability of the Ect2 system[2]. With this choice of $k_{\text{Cdk1}}(\mathbf{x}, t)$, we assume that the nucleus is positioned at the left side of the oocyte, at $x_{\text{nucleus}} = -R$, thereby breaking the symmetry of the system.

*Optogenetic GEF.* In addition to the native GEFs, optogenetic GEFs were introduced to the oocytes to make them sensitive to the applied illumination. In total, three different variants of the optogenetic complexes were used: (i) Opto-Null, not

| Symbol | Value | Description |
|---|---|---|
| $D_\text{E}$ | $10\ \mu\text{m}^2\,\text{s}^{-1}$ | Diffusion constant in the cytosol |
| $D_\text{e}$ | $0.5\ \mu\text{m}^2\,\text{s}^{-1}$ | Diffusion constant on the membrane |
| $k_\text{dp}$ | $2.5\ \text{s}^{-1}$ | Dephosphorylation rate |
| $k_\text{fb}$ | $0.5\ \mu\text{m}^2\,\text{s}^{-1}$ | Autocatalytic dephosphorylation rate |
| $K_\text{p}$ | $0.1\ \mu\text{m}^{-2}$ | Phosphorylation saturation constant |
| $k_\text{on,e}$ | $0.5\ \mu\text{m}\,\text{s}^{-1}$ | Ect2 membrane attachment |
| $k_\text{off,e}$ | $5\ \text{s}^{-1}$ | Ect2 membrane detachment |
| $k_{\text{Cdk1},0}$ | $100\ \text{s}^{-1}\,\mu\text{m}^{-2}$ | Reference phosphorylation rate |
| $\alpha_\text{Cdk1}$ | $3.6\ \text{s}^{-1}\,\mu\text{m}^{-3}$ | Cdk1 gradient slope |
| $\tau_\text{Cdk1}$ | $100\ \text{s}$ | Cdk1 decay time scale |
| $R$ | $100\ \mu\text{m}$ | Oocyte radius |
| $\bar{u}_\text{E}$ | $14.67\ \mu\text{m}^{-2}$ | (Total) average Ect2 concentration |

**Table S1** | List of parameters and their default values used for modeling the reaction-diffusion dynamics of the native GEF, Ect2.

containing a domain to catalyze the Rho nucleotide exchange; (ii) Opto-GEF, containing the catalyzing domain from the native Ect2 enzyme; and (iii) Opto-GEF*, containing the catalyzing domain from the exogenous LARG enzyme. Since the endogenous Ect2 and the exogenous LARG may interact differently with other proteins in the cell, there may be subtle differences in the reaction-diffusion dynamics. For example, the catalyzing domain of Ect2 is affected by phosphorylation mediated by Cdk1[4], which may not be the case for the LARG enzyme. Similarly, the enzymatic activity of both GEF variants (and thus their interaction with Rho, see below) might be different.

As discussed previously, the qualitative dynamics (guided waves, trigger waves, and pinches) are fairly robust to parameter variations, and variations in one parameter can often be compensated by variations in a number of other parameters. Notably, this includes the total concentration of optogenetic GEFs, which is determined by the expression level and is difficult to control experimentally, as well as cell-to-cell variations in other protein concentrations. Therefore, we will account for these variations by varying a single representative parameter, instead of fine-tuning all parameters to match all experimental conditions. In particular, we assume for simplicity that Opto-GEF and Opto-GEF* behave identically, and that Opto-Null obeys the same reaction-diffusion dynamics but does not contribute to the Rho nucleotide exchange. In this section, we therefore refer to all three optogenetic complex variants as Opto-GEF for brevity.

Disregarding all interactions with other proteins, the Opto-GEF dynamics are governed by photoactivation and membrane binding, where only photoactivated proteins can bind to the membrane. We therefore distinguish between three states of Opto-GEF: active and inactve Opto-GEF in the cytosol ($u_\text{Ga}$ and $u_\text{G}$, respectively) and membrane-bound Opto-GEF $u_\text{g}$ which is always in the active state. Similar to the native Ect2, the relevant set of partial differential equations is

$$\partial_t u_\text{Ga} = D_\text{G}\nabla^2 u_\text{Ga} + f_\text{Ga}(u_\text{Ga}, u_\text{G}), \tag{11}$$

$$\partial_t u_\text{G} = D_\text{G}\nabla^2 u_\text{G} + f_\text{G}(u_\text{Ga}, u_\text{G}), \tag{12}$$

$$\partial_t u_\text{g} = D_\text{g}\nabla^2_\mathcal{S} u_\text{g} + f_\text{g}\big(u_\text{Ga}|_\mathcal{S}, u_\text{G}|_\mathcal{S}, u_\text{g}\big). \tag{13}$$

$D_\text{G}$ and $D_\text{g}$ are the Opto-GEF diffusion constants in the cytosol and on the membrane, respectively. Under blue light illumination, the photosensitive domain of the Opto-GEF complexes is activated at a rate $k_\text{a}\cdot I(\mathbf{x},\, t)$, which enables them to bind to membrane anchors. Since the conformational change is induced by photon absorption, it is reasonable to assume that activation is proportional to the light intensity $I(\mathbf{x},\, t)$. Domains deactivate spontaneously at a rate $k_\text{d}$, independent of any applied illumination. Photoactivated Opto-GEF can bind to membrane-bound anchor domains (relative concentration around the mean distribution given by $u_a(\mathbf{x})$) at a rate $k_\text{on,g}$ and unbind at a rate $k_\text{off,g}$. This gives rise to the following reaction terms:

$$f_\text{Ga}(u_\text{Ga}, u_\text{G}) = I\cdot k_\text{a}\, u_\text{G} - k_\text{d}\cdot u_\text{Ga}\,, \tag{14}$$

$$f_\text{G}(u_\text{Ga}, u_\text{G}) = -I\cdot k_\text{a}\, u_\text{G} + k_\text{d}\cdot u_\text{Ga}\,, \tag{15}$$

$$f_\text{g}\big(u_\text{Ga}|_\mathcal{S}, u_\text{G}|_\mathcal{S}, u_\text{g}\big) = u_\text{a}\cdot k_\text{on,g}\, u_\text{Ga}|_\mathcal{S} - k_\text{off,g}\, u_\text{g}\,, \tag{16}$$

Similar to the Ect2 dynamics, we use no-flux boundary conditions for the inactive Opto-GEF, and reactive boundary

| Symbol | Value | Description |
|---|---|---|
| $D_\text{G}$ | $1\ \mu\text{m}^2\,\text{s}^{-1}$ | Diffusion constant in the cytosol |
| $D_\text{g}$ | $0.01\ \mu\text{m}^2\,\text{s}^{-1}$ | Diffusion constant on the membrane |
| $k_\text{a}$ | $7.5\cdot 10^{-2}\ \text{s}^{-1}$ | Photoactivation rate |
| $k_\text{d}$ | $6.7\cdot 10^{-4}\ \text{s}^{-1}$ | Photodeactivation rate |
| $k_\text{on,g}$ | $9\cdot 10^{-4}\ \mu\text{m}\,\text{s}^{-1}$ | Opto-GEF membrane attachment |
| $k_\text{off,g}$ | $9.2\cdot 10^{-4}\ \text{s}^{-1}$ | Opto-GEF membrane detachment |
| $\alpha_\text{a}$ | $0.5$ | Anchor gradient slope |
| $\bar{u}_\text{R}$ | $60\ \mu\text{m}^{-2}$ | (Total) average Opto-GEF concentration |

**Table S2** | List of parameters and their default values used for modeling the Opto-GEF dynamics.

conditions for the photoactivated Opto-GEF:

$$D_\text{Ga}\,\hat{\mathbf{n}}_\mathcal{S}\cdot\nabla\,u_\text{Ga}|_\mathcal{S} = -u_\text{a}\cdot k_\text{on,g}\,u_\text{Ga}|_\mathcal{S} + k_\text{off,g}\,u_\text{g}\,, \tag{17}$$

$$D_\text{G}\,\hat{\mathbf{n}}_\mathcal{S}\cdot\nabla\,u_\text{G}|_\mathcal{S} = 0\,. \tag{18}$$

At the beginning of each simulation, all Opto-GEF is assumed to be in the inactive state.

As discussed in Supplementary Information Section 1, the membrane CIBN/CaaX anchor complexes are expressed together with the photosensitive Opto-GEF during preparation of the oocytes. Afterwards, the anchor complexes bind on to the membrane. Intriguingly, we observed that the distribution of anchors across the oocyte membrane is not fully homogeneous, but there is a concentration gradient from the vegetal pole to the animal pole (Extended Data Fig. 6d). We propose that this asymmetric anchor distribution arises from the specific membrane interaction of the anchor complexes and volume exclusion by the nucleus. Prior to the membrane binding, the anchor complexes undergo post-translational modifications in the endoplasmatic reticulum[5]. Due to the asymmetric position of the nucleus, the AP side of the oocyte is partially shielded from the membrane-binding anchor complexes and complexes are more likely to encounter the VP side, resulting in a heterogeneous distribution of membrane anchors. Upon encountering the membrane, the CIBN/CaaX complexes effectively bind permanently to the membrane, with a detachment rate that is negligible on the time scale of observation. In addition, the anchor complexes can be considered to be immobile on the membrane due to low diffusion. This means that the process of membrane binding and the final distribution of anchors on the membrane can be interpreted as a first-passage-time problem[6]. In this context, proteins are more likely to encounter the membrane at the VP than at the AP, since the nucleus located at the AP is an obstacle that blocks a significant fraction of anchors from reaching the AP.

We account for this anchor gradient only when it is needed as a symmetry-breaking cue, i.e., when studying homogeneous global light activation. Otherwise, we use a homogeneous concentration to avoid side effects on the dominant dynamics, in particular for trigger waves:

$$u_\text{a}(\mathbf{x}) = 1 + \alpha_\text{a}\,x/R\,. \tag{19}$$

Here, $\alpha_\text{a}$ represents the slope of the gradient, and again, the nucleus is positioned at the left side of the oocyte. The impact of the anchor gradient on trigger waves and the oocyte's response to local illumination is discussed in Section 5.

For the light illumination, we use various expressions for $I(\mathbf{x},\,t)$ to represent different experimental realizations. To emulate pinching, we use a light pulse localized to one or multiple small regions of interest. To emulate fast traveling waves, we use a global light pulse. We also use more sophisticated illumination patterns for spatiotemporal deformation guidance.

$$\text{Pinch:}\qquad I(\mathbf{x},\,t) = \mathcal{T}(t)\cdot\sum_i \mathcal{R}(\mathbf{x}-\mathbf{x}_i)\,, \tag{20}$$

$$\text{Fast wave:}\qquad I(\mathbf{x},\,t) = \mathcal{T}(t)\cdot 1\,, \tag{21}$$

$$\text{Sequential pinch:}\qquad I(\mathbf{x},\,t) = \mathcal{T}(t)\cdot\mathcal{R}(\mathbf{x}-\mathbf{x}_1) + \mathcal{T}(t-T_\text{delay})\cdot\mathcal{R}(\mathbf{x}-\mathbf{x}_2)\,. \tag{22}$$

(23)

The index $i$ indicates the position of distinct regions of interest. Here, $\mathcal{T}(t)$ and $\mathcal{R}(\mathbf{x})$ are rectangular functions in space

| Symbol | Value | Description |
|---|---|---|
| $T_{\text{pulse}}$ | $10$ s | Duration of an illumination pulse |
| $T_{\text{circle}}$ | $3 \cdot 10^3$ s | Duration of one revolution around the oocyte |
| $T_{\text{delay}}$ | $9 \cdot 10^2$ s | Time between two sequential pinches |
| $d_{\text{ROI}}$ | $20\ \mu$m | Width of the illuminated region of interest |

**Table S3** | List of parameters and their default values used to vary the light illumination.

and time, respectively, defined by:

$$\mathcal{T}(t) = \begin{cases} 1 & \text{for} \quad 0 \leq t \leq T_{\text{pulse}} \,, \\ 0 & \text{else,} \end{cases} \tag{24}$$

$$\mathcal{R}(\mathbf{x}) = \begin{cases} 1 & \text{for} \quad \|\mathbf{x}\|_\infty \leq \frac{d_{\text{ROI}}}{2} \,, \\ 0 & \text{else.} \end{cases} \tag{25}$$

*Rho.* The native Ect2 and the optogenetic GEF, as well as potentially other GEFs that are not modeled explicitly, contribute to the conversion of Rho-GDP to Rho-GTP on the membrane. Previous work on wild-type SCWs suggested a model for the Rho-GTP dynamics that we adopt and expand here[2]. We distinguish between three different states of the Rho protein. In the cytosol, Rho is assumed to be always in the Rho-GDP state ($u_{\text{R}}$). On the membrane, Rho can be in the Rho-GDP ($u_{\text{rd}}$) or in the Rho-GTP state ($u_{\text{rt}}$). Thus, the reaction-diffusion equations read

$$\partial_t u_{\text{R}} = D_{\text{R}} \nabla^2 u_{\text{R}} \,, \tag{26}$$

$$\partial_t u_{\text{rd}} = D_{\text{rd}} \nabla^2_{\mathcal{S}} u_{\text{rd}} + f_{\text{rd}}\big(u_{\text{R}}|_{\mathcal{S}}, u_{\text{rd}}, u_{\text{rt}}\big) \,, \tag{27}$$

$$\partial_t u_{\text{rt}} = D_{\text{rt}} \nabla^2_{\mathcal{S}} u_{\text{rt}} + f_{\text{rt}}\big(u_{\text{R}}|_{\mathcal{S}}, u_{\text{rd}}, u_{\text{rt}}\big) \,. \tag{28}$$

For the reaction terms, we consider Rho-GDP binding to and unbinding from the membrane ($k_{\text{on,r}}$ and $k_{\text{off,R}}$, respectively). On the membrane, Rho-GDP is converted to Rho-GTP by any compatible GEF at a fixed rate $k_{\text{r}}$. The total GEF concentration is denoted by $u_{\text{e0}} = u_{\text{e}} + u_0$, where $u_{\text{e}}$ is the native Ect2 concentration on the membrane and $u_0$ corresponds to other GEFs that are not modeled explicitly. Note that the enzymatic activity of the various GEFs might be different, i.e., the rate $k_{\text{r}}$ should be seen as an effective rate. For the optogenetic GEFs ($u_{\text{g}}$) containing only the catalyzing DH domain, we assume linear Rho activation at a rate $k_{\text{rg}}$.

In addition to linear conversion from Rho-GDP to Rho-GTP, it is known that Rho-GTP can autocatalytically enhance Rho activation, presumably by interacting with other GEFs[7]. However, to our best knowledge, the precise molecular mechanism by which this positive feedback is realized remains unclear, and previous studies used effective descriptions of the autocatalysis instead[2,8,9]. Here, we use a quadratic amplification of the nucleotide exchange at a rate $k_{\text{dt}}\, u_{\text{rt}}^2$, which has been used previously to model the wild-type surface contraction waves of meiotic starfish oocytes[2] and is a simplified version of a model used for studying spiraling Rho dynamics in starfish and frog oocytes[8,9]. We note that, in general, other nonlinear interactions may lead to similar Rho excitations[10].

Finally, Rho-GTP is hydrolyzed to Rho-GDP and immediately detaches from the membrane at a rate $k_{\text{gap}}$. With this, the reaction terms for the Rho system read

$$f_{\text{R}}\big(u_{\text{R}}\big) = 0 \,, \tag{29}$$

$$f_{\text{rd}}\big(u_{\text{R}}|_{\mathcal{S}}, u_{\text{rd}}, u_{\text{rt}}\big) = k_{\text{on,r}}\ u_{\text{R}}|_{\mathcal{S}} - k_{\text{off,R}}\, u_{\text{rd}} - u_{\text{e0}} \cdot (k_{\text{r}} + k_{\text{dt}}\, u_{\text{rt}}^2)\, u_{\text{rd}} - u_{\text{g}} \cdot k_{\text{rg}}\, u_{\text{rd}} \,, \tag{30}$$

$$f_{\text{rt}}\big(u_{\text{R}}|_{\mathcal{S}}, u_{\text{rd}}, u_{\text{rt}}\big) = u_{\text{e0}} \cdot (k_{\text{r}} + k_{\text{dt}}\, u_{\text{rt}}^2)\, u_{\text{rd}} + u_{\text{g}} \cdot k_{\text{rg}}\, u_{\text{rd}} - k_{\text{gap}}\, u_{\text{rt}} \,. \tag{31}$$

The cytosolic Rho dynamics are subject to the boundary condition

$$D_{\text{R}}\, \hat{\mathbf{n}}_{\mathcal{S}} \cdot \nabla\, u_{\text{R}}|_{\mathcal{S}} = -k_{\text{on,r}}\ u_{\text{R}}|_{\mathcal{S}} + k_{\text{off,R}}\, u_{\text{rd}} + k_{\text{gap}}\, u_{\text{rt}} \,. \tag{32}$$

*Passive effect of optogenetic GEF.* The introduction of optogenetic GEFs to the starfish oocytes allows to trigger localized increases in the membrane-bound GEF concentrations by light illumination. However, the optogenetic constructs may also have a passive effect on the oocytes, i.e., an effect on the Rho dynamics even without illumination. The origin of this passive effect, however, has not yet been fully understood and cannot be determined unambiguously from our mesoscopic

| Symbol | Value | Description |
|---|---|---|
| $D_{\mathrm{R}}$ | $10\ \mu\mathrm{m}^2\,\mathrm{s}^{-1}$ | Rho-GDP diffusion constant in the cytosol |
| $D_{\mathrm{rd}}$ | $0.1\ \mu\mathrm{m}^2\,\mathrm{s}^{-1}$ | Rho-GDP diffusion constant on the membrane |
| $D_{\mathrm{rt}}$ | $0.1\ \mu\mathrm{m}^2\,\mathrm{s}^{-1}$ | Rho-GTP diffusion constant on the membrane |
| $k_{\mathrm{on,r}}$ | $1.5 \cdot 10^{-4}\ \mu\mathrm{m}\,\mathrm{s}^{-1}$ | Rho-GDP membrane attachment |
| $k_{\mathrm{off,R}}$ | $1.5 \cdot 10^{-5}\ \mathrm{s}^{-1}$ | Rho-GDP membrane detachment |
| $k_{\mathrm{r}}$ | $6.0 \cdot 10^{-4}\ \mu\mathrm{m}\,\mathrm{s}^{-1}$ | Effective nucleotide exchange rate (native) |
| $k_{\mathrm{rg}}$ | $6.0 \cdot 10^{-4}\ \mu\mathrm{m}\,\mathrm{s}^{-1}$ | Effective nucleotide exchange rate (Opto-GEF) |
| $k_{\mathrm{dt}}$ | $3.6 \cdot 10^{-2}\ \mu\mathrm{m}^3\,\mathrm{s}^{-1}$ | Effective autocatalytic nucleotide exchange rate |
| $k_{\mathrm{gap}}$ | $1.5 \cdot 10^{-2}\ \mathrm{s}^{-1}$ | Rho-GTP hydrolysis rate |
| $u_0$ | $0.3\ \mu\mathrm{m}^{-1}$ | Background GEF concentration |
| $\bar{u}_{\mathrm{R}}$ | $0.28\ \mu\mathrm{m}^{-2}$ | (Total) average Rho concentration |

**Table S4** | List of parameters and their default values used for modeling the Rho dynamics.

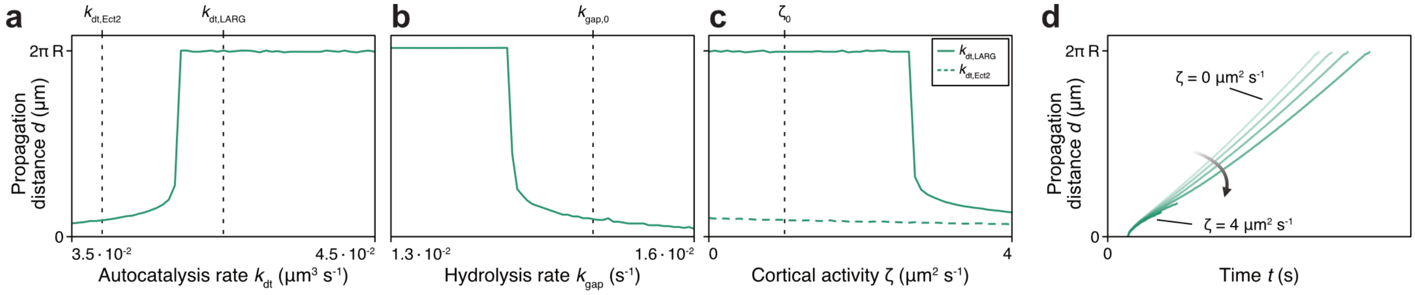


**Supplementary Fig. S4** | Transition between localized and propagating excitations, quantified by the simulated propagation distance of a Rho excitation after regional illumination. **a,** Propagation distance for varying autocatalysis rate $k_{\mathrm{dt}}$. The default values used in simulations for the Opto-GEF (Ect2) and the Opto-GEF* (LARG) cases are highlighted by dashed lines. **b,** A similar transition can be achieved by decreasing the hydrolysis rate $k_{\mathrm{gap}}$ below the default value $k_{\mathrm{gap,0}}$. **c,** Cortical contractions counteract the propagation of Rho exciations. For unguided waves as observed for Opto-GEF* (solid line), sufficiently strong cortical activity is expected to result in pinch deformations rather than waves. In contrast, pinch deformations as observed for Opto-GEF (dashed line) cannot be transformed to unguided waves by decreasing the cortical activity. **d,** Propagation distance of the Rho peak over time for increasing cortical activity $\zeta$ (indicated by arrow), simulated using the Opto-GEF* autocatalysis rate $k_{\mathrm{dt,LARG}}$. Increasing the activity initially slows down the wave until the transition to pinch-like phenotypes occurs.

experiments. In Section 4.4, we provide a detailed discussion of the supporting experimental evidence for this passive effect, as well as the possible mechanism based on our theoretical analysis. In general, the prolonged cortical activity in Opto-GEF*-expressing meiotic oocytes and the facilitated propagation of unguided Rho excitations in photoactivated oocytes hint towards an effect on the nonlinear Rho dynamics, since the autocatalytic Rho activation lies at the heart of both processes. In simulations, we therefore realize the passive difference between Opto-GEF and Opto-GEF* by modulating the effective autocatalytic nucleotide exchange rate $k_{\mathrm{dt}}$. Importantly, increasing $k_{\mathrm{dt}}$ is sufficient to transition from a localized pinch deformation to an unguided SCW after regional illumination (Fig. S4a). However, we note that similar transitions can be observed by varying other parameters, such as the hydrolysis rate $k_{\mathrm{gap}}$ (Fig. S4b), and our choice of varying the autocatalysis rate is but one out of multiple options how Opto-GEF* could passively affect the Rho dynamics.

*Advective membrane flows.* The cortical response to high Rho-GTP concentration is known to not only cause geometry deformations but also in-plane contractile flows of the cortex[11]. The cortex is hydrodynamically coupled to both the cell membrane and the cytoplasm, and thus generically cortical flows also cause cytoplasmic flows and membrane flows[12]. The former have been observed in previous studies of the starfish oocyte's SCWs[11] and are also observed in our experiments (Extended Data Fig. 9a,b). For local activation, these cytoplasmic flows that form near the illuminated region can also be detected via PIV analyses (Methods) upon a few seconds of illumination (data not shown). However, since the decisive protein interactions (in particular the nonlinear feedback) take place on the membrane, membrane flows may have a much more relevant role for the propagation of SCWs, and therefore we will focus on those flows.

In the context of pattern formation coupled to advective flows, Mayer et al. have derived a description based on active fluids[13,14] which has been successfully implemented to study cortical tension in the *C. elegans* zygote[15]. Here, we adopt the same formalism assuming that the membrane flows are directly coupled to the cortical flows. The constitutive relation

for the flow velocity $\vec{v}$ is then

$$\frac{1}{\ell}\,\vec{v} = \nabla_{\mathcal{S}}\, C_0\, \chi(u_{\text{rt}}) + \ell\, \nabla_{\mathcal{S}}\big(\nabla_{\mathcal{S}} \cdot v\big)\,, \tag{33}$$

where $\ell$ is a correlation length scale of advective fluxes and $C_0 = \zeta/\ell$ is the maximum contractility of the cortex with the effective actomyosin activity $\zeta$. We assume that Rho-GTP directly causes cortex contractions rather than modeling the actin and myosin dynamics explicitly, i.e.,

$$\chi(u_{\text{rt}}) = \tanh\left(\frac{u_{\text{rt}}}{u_{\text{rt},0}}\right)\,. \tag{34}$$

Note that other similar saturating expressions for the contractility, in particular using a Monod relation $\chi(u_{\text{rt}}) \sim u_{\text{rt}}/(u_{\text{rt}} + u_{\text{rt},0})$, produce equivalent results. Including the advection velocity $\vec{v}$ the PDEs for the membrane concentration fields then read

$$\partial_t u_i = \nabla_{\mathcal{S}}\big(D_i\, \nabla_{\mathcal{S}}\, u_i - \vec{v} \cdot u_i\big) + f_i\,. \tag{35}$$

The effect of advective flows in the membrane on the Rho dynamics (and thus on the shape deformations) for varying contractility strengths $\zeta$ is shown in Fig. S4c,d. In fact, the advection is only relevant for the propagation of unguided trigger waves: these waves progress because net diffusive Rho-GTP fluxes at the wave front increase the Rho-GTP concentration in neighbouring regions (state perturbations), thereby causing an excitation in the neighbourhood. Contractile flows, on the other hand, lead to fluxes towards high concentrations of Rho-GTP and thus counteract the diffusive fluxes. Consequently, the state perturbations in neighbouring regions is decreased as the strength of the contraction increases, and excitations become less pronounced. On the scale of the oocyte, this means that trigger waves may not travel across the entire circumference of the oocyte but decay early. In other words, advective membrane flows decrease state perturbations. However, since the effect of advection can be balanced by increasing the state perturbations by other means (e.g., by varying the parameters of the nonlinear feedback) or by globally lowering the excitation threshold (e.g., by changes in the concentration of endogenous GEFs), it is not possible to observe this effect directly in experiments. Most importantly, within the scope of our analysis, the spectrum of deformation phenotypes is independent of the presence of advective flows.

#### Simulations of the mechanical module

In the mechanical module, we couple the Rho-GTP dynamics obtained from the chemical module to a deformable surface to reconstitute the oocyte deformations in simulations. The corresponding partial differential equation was solved numerically using Wolfram Mathematica 13.1. In agreement with the chemical module, we simulate a slice of the oocyte as a representation of the full (three-dimensional) oocyte.

To simulate the shape dynamics, we model the oocyte membrane and cortex as a single elastic surface whose shape is governed by surface tension-like contraction and bending rigidity. Contractions and the resistance against stretching originate in the actomyosin activity in the cortex[16]. Enhanced actomyosin activity is triggered by the presence of Rho-GTP[17]. Recently, the pattern-forming properties of actomyosin activity and its promoters (Rho-GTP for the starfish oocytes) have been studied, where it was shown that to lowest order the actomyosin activity follows the concentration of the promoter[18]. To focus on the connection between the Rho dynamics and the deformations, rather than accounting for the explicit actomyosin dynamics, we therefore approximate the actomyosin activity as a function of the Rho-GTP concentration $\chi(u_{\text{rt}})$. Here,

$$\chi(u_{\text{rt}}) = \tanh\left(\frac{u_{\text{rt}}}{u_{\text{rt},0}}\right) \tag{36}$$

is linear in $u_{\text{rt}}$ at low Rho-GTP concentrations and saturates at high Rho-GTP concentrations, with a saturation concentration $u_{\text{rt},0}$. The actomyosin activity is assumed to cause local contractions, modeled as a surface tension-like term in an effective free energy functional with strength $\lambda$. Strong local deformations are counteracted by the bending rigidity $\kappa$ of the cortex.

Both contributions (contractions and bending rigidity) give rise to the following free energy functional:

$$\mathcal{H}\big[r(\theta), u_{\text{rt}}(\theta)\big] = \int_0^{2\pi} \mathrm{d}\theta\, \sqrt{g}\, \left[\lambda\, \chi(u_{\text{rt}}(\theta)) + \frac{\kappa}{2}\left(\frac{r^2 + 2\,(\partial_\theta r)^2 - r\,\partial_\theta^2 r}{\sqrt{g}^3} - H_0\right)^2\right]\,. \tag{37}$$

The determinant of the metric $g = r(\theta)^2 + (\partial_\theta r(\theta))^2$ accounts for the arc length of the oocyte surface in polar coordinates, and $r(\theta)$ is the radius of the cell. $H_0$ is the preferred curvature of the surface, which is taken to be the inverse of the unperturbed oocyte's radius, $H_0 = 1/R$.

To obtain the time evolution of the oocyte shape, we assume relaxational dynamics of the surface towards the minimum of the effective free energy with a characteristic time scale $\tau$. In addition to the contributions described above, the oocytes

| Symbol | Value | Description |
|---|---|---|
| $u_{\text{rt},0}$ | $15\ \mu\text{m}^{-1}$ | Rho-GTP saturation concentration |
| $\lambda$ | | Surface contraction strength |
| $\kappa$<br>$\kappa/\lambda$ | <br>5 | Bending rigidity |
| $H_0$ | $10^{-2}\ \mu\text{m}^{-1}$ | Preferred curvature ($= 1/R$) |
| $\tau$<br>$\tau/\lambda$ | <br>$1\ \text{s}\,\mu\text{m}^{-2}$ | Relaxation time scale |
| $\tau_{\text{Area}}$ | $2\pi\,10^2\ \text{s}\,\mu\text{m}^{-2}$ | Area conservation time scale |
| $\ell$ | $15\ \mu\text{m}$ | Correlation length scale of advective fluxes |
| $\zeta$ | $1\ \mu\text{m}^2\,\text{s}^{-1}$ | Effective cortical activity |

**Table S5** | List of parameters and their default values used for modeling the shape dynamics.

are subject to volume conservation. In our 2D projection, this corresponds to a conservation of the oocyte area

$$A = \frac{1}{2}\int_0^{2\pi} \mathrm{d}\theta\, r^2(\theta)\,. \tag{38}$$

This conservation law is implemented as a soft constraint with a characteristic time scale $\tau_{\text{Area}}$, where the target area is identical to the initial area $\pi\, R^2$. Altogether, we obtain the following partial differential equation for the oocyte radius $r(\theta, t)$:

$$\partial_t r(\theta,t) = -\frac{1}{\tau}\frac{\delta\mathcal{H}\big[r, u_{\text{rt}}\big]}{\delta r} + \frac{1}{\tau_{\text{Area}}}\cdot 2\,r\left(1 - \frac{1}{\pi\, R^2}\cdot\frac{1}{2}\int_0^{2\pi}\mathrm{d}\theta\, r^2\right) \tag{39}$$

with initial condition $r(\theta, 0) = R$. To improve numerical efficiency, the oocyte area is only updated at discrete time intervals of $\Delta t = 10\,\text{s}$.

To simulate the deformation response of an oocyte to a light stimulus or the native guiding cue (Cdk1), we first solved the chemical reaction-diffusion dynamics as described above. From this, the Rho-GTP concentration $u_{\text{rt}}$ on the oocyte surface was obtained for the entire simulated time. In a subsequent step, we derived the time-dependent approximated actomyosin activity $\chi\big(u_{\text{rt}}(\theta,t)\big)$ and simulated the oocyte deformation as described above.

## 3 Excitation threshold and activation

The observed deformation dynamics are rooted in the the spatio-temporal Rho-GTP dynamics and in particular the Rho-GTP excitations[11]. For a spatially homogeneous system the Rho-GTP excitations can be visualized conveniently in terms of a phase portrait. Making use of the mass conservation of the Rho system and disregarding any gradients in the cytosol, one can eliminate the cytosolic Rho concentration and represent the state of the system in terms of the concentrations of Rho-GDP and Rho-GTP on the membrane (Fig. S5a). Previous work showed that a sudden change in the GEF concentration changes the shape of the phase portrait. Thereby, a state that was close to a stable fixed point before the GEF concentration changed can suddenly be far away from the shifted fixed point, leading to a Rho-GTP excitation (Fig. S5a). For such a homogeneous system, the impact of all model parameters on the dynamics can easily be examined by studying their effect on the phase portrait[2].

In the case of light-sensitive starfish oocytes a representation of the Rho dynamics in terms of a phase portrait is no longer appropriate. Whether and when a Rho-GTP excitation takes place at a specific point on the membrane depends on various factors, including the total Rho concentration, the local GEF concentration dynamics (native GEFs and optogenetic GEF), the Rho-GTP concentration in the neighbouring membrane regions and the history of the system. All of these factors lead to a spatial and temporal heterogeneity of the Rho system on the membrane. To extend the aforementioned parameter analysis to this case, the phase portrait would need to be extended by dedicated axes for the spatial and temporal variation, which is arguably difficult to visualize and interpret. A different representation is therefore needed to quantitatively analyze the Rho dynamics.

### Excitation threshold

In the case of a spatio-temporally varying environment, the phase portrait carries more information than could be useful. In fact, if an explicit numerical solution of the entire dynamics should be avoided, the relevant information is contained in the local and instantaneous phase space trajectory of the system. Here, the terms "local" and "instantaneous" refer to a

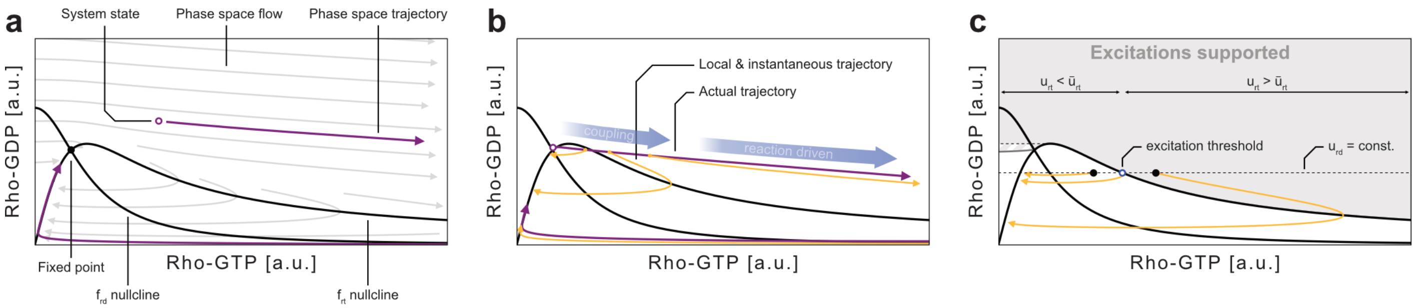


**Supplementary Fig. S5 | Phase portrait analysis and excitation threshold. a,** Characteristic phase portrait of the Rho reaction network. Black lines indicate the $f_{\mathrm{rt}}$ and $f_{\mathrm{rd}}$ nullclines. Gray lines indicate the phase space flow, and the purple line represents a specific trajectory in this phase portrait given a specific system state as initial condition. **b,** In a spatially extended system, diffusive coupling can affect the position of a system in phase space. The purple line corresponds to a (simulated) trajectory which is carried away from the stable fixed point due to diffusive coupling initially, whereas reactions lead to an excitation afterwards. Orange lines are phase space trajectory originating from selected states on the simulated trajectory (purple). **c,** Construction of the excitation threshold: on a subspace of constant $u_{\mathrm{rd}}$, the excitation threshold lies on the intersection with the $f_{\mathrm{rt}}$ nullcline. Only if $u_{\mathrm{rt}} > \bar{u}_{\mathrm{rt}}$, excitations are possible (orange lines). The shaded area indicates regions where excitations are supported.

phase portrait constructed for parameters and concentrations at a specific point in space and time, explicitly disregarding that this phase portrait might change in a subsequent time step. This local and instantaneous trajectory is therefore an approximation of the actual trajectory that the system will follow (Fig. S5b).

For deforming starfish oocytes, this information can be reduced even further. To observe a deformation, a Rho-GTP excitation is needed, but the actual shape of the trajectory in phase space is less relevant. Thus, it is instructive to ask whether the phase space trajectory, at a given point in space and time, corresponds to an excitation (i.e., reactions drive the system further away from the stable fixed point) or a relaxation towards a stable fixed point. This property of the trajectory is determined by the system state relative to the nullclines, in particular the nullcline pertaining to the excitable quantity (Rho-GTP for starfish oocytes). The Rho-GTP nullcline is the curve in $(u_{\mathrm{rt}}, u_{\mathrm{rd}})$-space for which the Rho-GTP reaction term is zero, $f_{\mathrm{rt}}\big(u_{\mathrm{R}}|_{\mathcal{S}}, u_{\mathrm{rd}}, u_{\mathrm{rt}}\big) = 0$. By solving this equation for $u_{\mathrm{rd}}$, the nullcline can be expressed as

$$u_{\mathrm{rd,nc}}(u_{\mathrm{rt}}) = \frac{k_{\mathrm{gap}}\, u_{\mathrm{rt}}}{u_{\mathrm{e0}}(k_{\mathrm{r}} + k_{\mathrm{dt}}\, u_{\mathrm{rt}}^2)} \,. \tag{40}$$

For a local and instantaneous phase portrait, the cytosolic Rho-GDP concentration $u_{\mathrm{R}}|_{\mathcal{S}}$ can be eliminated assuming mass conservation. In the following, we account for the mass conservation implicitly by defining reaction terms in $(u_{\mathrm{rt}}, u_{\mathrm{rd}})$-space as

$$\bar{f}_{\mathrm{rt}}(\mathbf{u}) = f_{\mathrm{rt}}\left(n_{\mathrm{R}} - \tfrac{2}{R}(u_{\mathrm{rd}}{+}u_{\mathrm{rt}}), u_{\mathrm{rd}}, u_{\mathrm{rt}}\right) \,, \tag{41}$$

$$\bar{f}_{\mathrm{rd}}(\mathbf{u}) = f_{\mathrm{rd}}\left(n_{\mathrm{R}} - \tfrac{2}{R}(u_{\mathrm{rd}}{+}u_{\mathrm{rt}}), u_{\mathrm{rd}}, u_{\mathrm{rt}}\right) \,. \tag{42}$$

Here, $n_{\mathrm{R}}$ corresponds to the total Rho-GTP mass (which is now a parameter for $\bar{f}_{\mathrm{rt,rd}}$) and the prefactor $2/R$ maps membrane concentrations to volume concentrations. In the specific case of the Rho system, the phase portrait structure allows to characterize almost all states as “excitable” or “relaxing” by the sign of the reaction term $\bar{f}_{\mathrm{rt}}$. As shown in Fig. S5c, the region where states are excitable overlaps largely with the region where $\bar{f}_{\mathrm{rt}} > 0$ except for a small region at low Rho-GTP concentrations.

The sign of the $\bar{f}_{\mathrm{rt}}$ rate serves as an approximate measure to identify whether a system is is making an excursion in phase space. In a subsequent step, we focus on states that are not (yet) on such an excursion trajectory. How would such a state need to be perturbed to become excitable? Any system in the relaxational region can be brought to the excitable region either by increasing the Rho-GTP or the Rho-GDP concentration. For two diffusively coupled membrane compartments, an excitation in one compartment will significantly increase the Rho-GTP concentration and slightly decrease the Rho-GDP concentration, and diffusion will cause similar but weakened effects in the neighbouring compartment. Since the Rho-GTP variation is strongest, we neglect the comparably small Rho-GDP concentration change and ask how much the Rho-GTP concentration needs to be increased in order to put the system on an excursion in phase space. To find the threshold in the Rho system, we construct an auxiliary subspace in the phase space defined by a simplex at constant Rho-GDP concentration $u_{\mathrm{rd}}$ (Fig. S5c). This subspace can intersect with the $\bar{f}_{\mathrm{rt}}$ nullcline, where we refer to the largest Rho-GTP concentration at an intersection as $\bar{u}_{\mathrm{rt}}$. Due to the specific phase portrait structure of the Rho reaction network, a system at a state $(u_{\mathrm{rt}}, u_{\mathrm{rd}})$ can be moved to the excitable region by increasing the Rho-GTP concentration by $\delta u_{\mathrm{rt}} > \bar{u}_{\mathrm{rt}} - u_{\mathrm{rt}}$. Therefore this Rho-GTP concentration $\bar{u}_{\mathrm{rt}}$ is an *excitation threshold* for a system that is not yet on an excursion in phase space[19,20].

Formally, this excitation threshold can be defined by calculating the intersection between the nullcline and the $u_{\mathrm{rd}}$ subspace which are given by

$$u_{\mathrm{rt},\pm} = \frac{k_{\mathrm{gap}} \pm \sqrt{k_{\mathrm{gap}}^2 - 4k_{\mathrm{dt}}\, k_{\mathrm{r}}\, u_{\mathrm{e0}}^2\, u_{\mathrm{rd}}^2}}{2k_{\mathrm{dt}}\, u_{\mathrm{e0}}\, u_{\mathrm{rd}}}\,, \tag{43}$$

where the excitation threshold is the largest value $\bar{u}_{\mathrm{rt}} = u_{\mathrm{rt},+}$. When there is no intersection between the subspace and the nullcline (i.e., for $u_{\mathrm{rd}} > \sqrt{k_{\mathrm{gap}}^2/(4\, k_{\mathrm{dt}}\, k_{\mathrm{r}}\, u_{\mathrm{e0}}^2)}$), the excitation threshold is taken to be $\bar{u}_{\mathrm{rt}} = 0$, since in this case all trajectories make an excursion in phase space irrespective of the Rho-GTP concentration. Using this definition, we identify a state $(u_{\mathrm{rt}}, u_{\mathrm{rd}})$ to lie on an excursion trajectory in phase space if

$$u_{\mathrm{rt}} > \bar{u}_{\mathrm{rt}}|_{u_{\mathrm{rt}}}$$

and relaxing towards the stable fixed point else. States that are relaxing towards the fixed point can be brought on an excursion in phase space by increasing the Rho-GTP concentration to values larger than the excitation threshold.

State perturbations and threshold perturbations.

The position of a state in phase space relative to the excitation threshold characterizes the local and instantaneous Rho reaction dynamics, and can be used to distinguish between excitation, relaxation, and oscillations. The theory of excitable media and the excitation threshold is well discussed in pertinent textbooks and reviews[20,21]. However, the distinction between the two different modes of excitation (state perturbations and threshold perturbations) is crucial for explaining the different observed phenotypes. Therefore, in the following, we will elaborate on these two different modes and discuss them in the context of the (optogenetically activated) Rho system.

*State perturbations.* First, we focus on how the spatial coupling of the Rho dynamics can lead to propagating and self-sustained excitations, commonly referred to as *trigger waves*[20,22,23]. For this, consider a situation where the Rho-GTP concentration on the membrane is inhomogeneous such that $\Delta_{\mathcal{S}} u_{\mathrm{rt}}(x) \neq 0$ almost everywhere. Consider a location $x_0$ on the membrane at the edge of a concentration peak (Fig. 3d-f), i.e., where $\Delta_{\mathcal{S}} u_{\mathrm{rt}}(x_0) > 0$. At this point on the membrane, the Rho-GTP concentration increases due to diffusive fluxes. Neglecting for simplicity the concentration gradients in the Rho-GDP concentration on the membrane and in the cytosol, this changes the phase space position of the system at $x_0$ along the $u_{\mathrm{rd}}(x_0)$-subspace. For subthreshold perturbations the chemical reactions counteract this Rho-GTP increase and drive the system back to the stable fixed point. However, for sufficiently strong diffusive fluxes $\nabla_{\mathcal{S}}^2 u_{\mathrm{rt}}(x_0) \gg -\bar{f}_{\mathrm{rt}}$ the Rho-GTP concentration can be increased across the excitation threshold (superthreshold perturbation). From that point on, the chemical reactions cause an excitation and further enhance the Rho-GTP increase at $x_0$. The ensuing transient concentration peak then causes subsequent excitations in susceptible neighbouring regions, allowing the excitation to spread through the medium as a trigger wave[20].

Since excitations in this situation are caused by diffusive fluxes from neighbouring membrane regions that change the local state of the system (position in phase space), we refer to this as *state perturbation*. The strength of the diffusive influxes determines the amplitude of the Rho-GTP peak in two different ways. First, the diffusive fluxes need to cause a superthreshold state perturbation, where stronger perturbations lead to stronger excitations. Second, the time over which the Rho-GTP mass increases needs to be sufficiently short to reduce the counteracting effect of the chemical reactions to the Rho-GTP increase in the initial subthreshold phase of the perturbation. Therefore, the effective strength of the state perturbation depends on the reaction rates and the GEF concentration, so that gradients in these rates or in $u_{\mathrm{e0}}$ can lead to a spatially varying response (which manifests itself in the Rho-GTP peak amplitude) along the oocyte membrane. Furthermore, propagating concentration waves decay when the state perturbations are too weak, giving rise to waves that only travel across a segment of the membrane or, in extreme cases, decay almost immediately.

*Threshold perturbations.* Now we focus on the response to temporally varying parameters, assuming a homogeneous protein distribution on the cell membrane at or close to the stable fixed point.

Before the parameter change, the excitation threshold $\bar{u}_{\mathrm{rt},0}$ is larger than the current Rho-GTP concentration. A sudden parameter change can shift this threshold significantly. In particular, an increase in the GEF concentration due to photoactivation can move the threshold below the current system state, which then again leads to an excitation. However, in contrast to the aforementioned state perturbations, this excitation is due to a change of the threshold. We therefore refer to this mechanism as *threshold perturbation*. Notably, the Rho-GTP excitations observed in wild-type oocytes[2,24] are caused by such threshold perturbations. Here, the Ect2 concentration changes very quickly at a point on the membrane when the Ect2 front passes by, corresponding to the sudden parameter change required for threshold perturbations.

The amplitude of the excitation depends on the position of the excitation threshold after the parameter change. When the threshold is close to the pre-perturbation system state $u_{\mathrm{rt},0}^*$, only a small peak will be observed, whereas the amplitude will be larger when the threshold becomes very small, possibly even zero. In combination with the state perturbations that cause trigger waves, the excitation amplitude following a threshold perturbation can have a significant impact on

the overall response: A small threshold perturbation may not lead to sufficiently strong state perturbations outside the illuminated region, so that no wave can be established, whereas a strong threshold perturbation may well kick off a robust trigger wave (Fig. 5e, Extended Data Fig. 8).

## 4 Experimental and modelling verification of proposed interactions

In this section, we discuss separate control experiments used to confirm essential aspects of the proposed chemo-mechanical feedback loop. In addition, we elaborate on the matching between experimental and simulation results.

### Rho

In experiments, the limited number of available photochannels poses two difficulties for the direct visualization of Rho GTPase activities that accompany light activation: Firstly, the Rho GTPase probe (rGBD reporter[25], Methods) is tagged by a GFP protein, thus the excitation photo channel coincides with the wavelength for photoactivation (488 nm); Secondly, the Rho GTPase probes are localized near the membranes, and thus need to be distinguished from the membrane anchor complex (CIBN-GFP, Methods), which also has a eGFP tag. Thus, we developed a separate control experiment where the CIBN-CaaX sequence was cloned into a fluorescence-untagged construct. The mRNA of the untagged anchor complex was then mixed with the mRNAs of both the Opto-GEF photosensitive construct and the Rho GTPase probe for protein expression in starfish oocytes. With these oocytes, we performed global activation experiments, such that the blue light stimulus can excite the Rho GTPase probe as well as activate the optical switch (Methods). We found that the kinetics of the probed Rho-GTP membrane density closely follows the rapid switch-on kinetics of Opto-GEF membrane accumulation (Extended Data Fig. 3a-b, Movie S2). In addition, we observed significant spatio-temporal fluctuations in the near-membrane Rho activity that are reminiscent of previously reported Rho oscillation dynamics[15] (Fig. 2d, Extended Data Fig. 3d, Movie S3). Together, this suggests an enhanced cortical excitability following light stimulation, consistent with the predicted effect of threshold perturbation via light activation.

### Myosin

*Myosin imaging.* To image myosin dynamics, we expressed fluorescently labeled non-muscle myosin II protein in starfish oocytes. Specifically, we chose to overexpress the GFP-tagged version of myosin II heavy chain protein (MHC-GFP, Methods). This is because existing research in meiotic starfish oocytes[26] has established that non-muscle myosin II is the major myosin species responsible for cortical contraction, and that the labeling of its heavy-chain component gives the best read-out for myosin cortical recruitment when compared to the essential or regulatory light chains. We verified this choice of myosin label by recording the time series of MHC-GFP-expressing starfish oocytes during meiosis (Extended Data Fig. 4a). Consistent with what was reported, we observed a traveling wave of cortical GFP signal recruitment that closely guides the change of local surface curvature (Extended Data Fig. 4b).

Next, we co-expressed this myosin label together with the light-inducible GEF recruitment assay (photo-recruitable Opto-GEF and GFP-free membrane anchor) in prophase-arrested starfish oocytes. Since the excitation wavelength of the GFP label coincides with the light activation wavelength (488 nm), we performed global light activation by capturing a first snapshot of assay-loaded oocytes in the GFP channel. To minimize photo-bleaching of the GFP label, we avoided continuous activation of the oocytes, but instead captured a second snapshot after another 10 min in dark (note that the optical switch has fast-on-slow-off kinetics). Indeed, when comparing the two snapshots, we observed a significant increase of cortical myosin that co-localizes with Opto-GEF accumulation after the global light activation (Extended Data Fig. 4c, left). Similar to what we reported in the original submission, such myosin recruitment is also spatially dictated by the enriched presence of membrane anchors at the vegetal pole (VP) and generates a prominent global deformation accordingly (Extended Data Fig. 4c, right).

When oocytes are subjected to continuous global activation, strong photo-bleaching effects make the retrieval of continuous myosin signals from this GFP label more difficult. Nevertheless, we observed that the time-lapse cortical enrichment of myosin closely accompanies the recruitment of Opto-GEF (Extended Data Fig. 4d). Taken together, we conclude that the myosin imaging experiments corroborate our assumption that light-induced GEF recruitment induces cell surface curvature changes via cortical recruitment of myosin II.

*Myosin inhibition.* We aimed to conduct myosin inhibition experiments post light activation to confirm that myosin activity is indeed essential for the light-induced surface contractions. However, a practical constraint is that blebbistatin, the sole functional inhibitor of non-muscle myosin II validated in starfish oocytes[26], is sensitive to blue light[27] and quickly loses effectiveness under the 488 nm illumination used to activate the Opto-GEF switch. Thus, to address the role of myosin activity, we designed and performed a new set of experiments. We were inspired by the reported uses of localized blebbistatin photo-inactivation to revert myosin II ATPase inhibition in acto-myosin contractility assays[28,29]. Since light-induced Opto-GEF activation recruits cortical myosin (as we showed in the myosin imaging experiments, Extended Data Fig. 4a-d), we predict that the light-induced blebbistatin inactivation restores activity of these recruited myosin and thus will further amplify the light-induced surface contractions.

We tested this prediction by generating two control variables, the global expression of Opto-GEF assay and the global blebbistatin treatment (200 $\mu$M, 2hr treatment, Methods), in the assay of four groups of oocytes: Group 1: no Opto-GEF assay expression, no prior blebbistatin inactivation; Group 2: no Opto-GEF, with blebbistatin; Group 3: with Opto-GEF, no blebbistatin; Group 4: with Opto-GEF, with blebbistatin. We next subjected these oocyte groups to identical procedures of local 488 nm illumination and compared their light-induced surface contraction responses (Extended Data Fig. 4e). We quantified these contractions by extracting the surface deformation rates – a metric that has been benchmarked in existing work[16] – and also verified in our set-up the inhibitory effect of blebbistatin (200 $\mu$M, 2 hr treatment) for meiotic surface contractions (Extended Data Fig. 4e, left). Consistent with our prediction, the control-variable experiment showed that both local activation of Opto-GEF (group 3) and local inactivation of blebbistatin (group 2) can independently induce a localized surface contraction (Extended Data Fig. 4e, right). When combined (group 4), the surface contraction response is significantly enhanced compared to groups 2 and 3 (Extended Data Fig. 4e, right).

Taken together, we conclude that in our light activation assays, myosin recruitment to the oocyte cortex closely follows light-induced recruitment of Opto-GEF and is responsible for the local surface contraction that we observed.

#### Opto-Null

For the Opto-GEF reaction-diffusion dynamics, we developed a model with linear reaction kinetics. The membrane binding and unbinding rates were determined through a separate control experiment using the Opto-Null assay: the membrane anchor paired with the mCherry-tagged photosensitive domain without the catalytic GEF domain (Methods). By performing pulsed and continuous global activation of oocytes expressing the control tag complex (Fig. 2b, Methods, Extended Data Fig. 3a,c), we gauged the binding kinetics for Opto-Null membrane recruitment, which we took as the same for Opto-GEF and Opto-GEF* as they share the same binding kinetics between the photosensitive domain and the membrane anchor. Next, we quantified the correlation of the Rho activity with the membrane-recruited Opto-GEF using local activation experiments of the fully functional variant of the optogenetic tag complex (Fig. 2c-d, Extended Data Fig. 3d-f). Since the optogenetic GEF only contains the catalytic DH domain, it is expected to contribute to the direct (linear) Rho nucleotide exchange in the same way as as the previously studied endogenous Ect2[2]. However, no autocatalytic activation is expected because the PH domain essential for autocatalytic Rho activation by Ect2[30] is cleaved. Assuming this linear interaction, we constructed a mathematical model linking arbitrary optical or cell-cycle dependent guiding cues to the Rho dynamics. Finally, in line with previous studies[17,18], the cortex contractility is assumed to depend directly on the Rho-GTP concentration. With this simplification, parameters for the mechanics of the cell cortex were estimated using the wild-type SCW assay (Section 2.2).

#### Opto-GEF*

The introduction of optogenetic GEFs to cells in principle can give rise to an indirect influence on the endogenous GEF-Rho excitability, for example if a small portion of the cytosolic optogenetic GEF expression mediates Rho catalytic activity at membrane[31]. Indeed, in recent work on light-induced furrow formation in HeLa cells, a photosensitive GEF based on the DH domain of the Leukemia-associated RhoGEF[32] (LARG) was reported to induce stress fiber formation without subjecting the cells with expression to light illumination[33,34]. This was interpreted as a ”passive effect” on Rho activity, which intriguingly was not present for the same cells using an Ect2 DH domain-based photosensitve GEF. Here, we adopt this phrasing of a ”passive effect” to describe a similar effect we found for both Ect2-based and LARG-based optogenetic GEF constructs, when they are expressed in prophase-arrested starfish oocytes without light activation. Intriguingly, similar to the observations in HeLa cells, we also found in our experiments that such a passive effect plays out more prominently for the optogenetic LARG-based construct (Opto-GEF*) compared to the optogenetic Ect2-based construct (Opto-GEF).

This observation comes from a separate control experiment we performed for meiotic oocyte behaviors with expression of Opto-GEF or Opto-GEF* assay in comparison to wild-type meiotic oocytes. We made use of the fact that an endogenous GEF wavefront sweeps from vegetal to animal pole in the anaphase of meiosis I[2] and that an amplified Rho excitation (due to the endogenous GEF wavefront) can cause drastic mechanical responses. In the absence of light activation, we subjected three groups of prophase-arrested starfish oocytes to hormone stimulus and induced their entry of meiotic cell cycle: (i) wild-type oocytes; (ii) oocytes with Opto-GEF assay (photo-recruitable Opto-GEF and membrane anchor) expression; (iii) oocytes with Opto-GEF* assay expression.

Surprisingly, we found the prominent presence of a signature ectopic phenotype (extreme deformations with subsequent lysis) in oocytes with high Opto-GEF* assay expression levels. Although no photo-activation is applied, the Opto-GEF* oocytes (group (iii)) exhibit a drastic elevation of surface contraction at the vegetal pole at the approximate time when the endogenous GEF wavefront is initiated at the vegetal pole (by comparison with wild-type oocytes in group (i)) (Extended Data Fig. 7e). This drastic contraction quickly leads to a shrink in the in-plane cell area and often results in subsequent cell lysis. In Opto-GEF oocytes (group (ii)), such a vegetal-pole elevation of surface contraction is also observed, however even at similarly high expression levels of the photo-recruitable construct (Opto-GEF vs Opto-GEF*), the elevation only causes a minor shrink and thus blebbing at the vegetal pole, and no lysis is observed (Extended Data Fig. 7e). These observations (Extended Data Fig. 7f) thus suggest that Opto-GEF* (under similar expression levels as

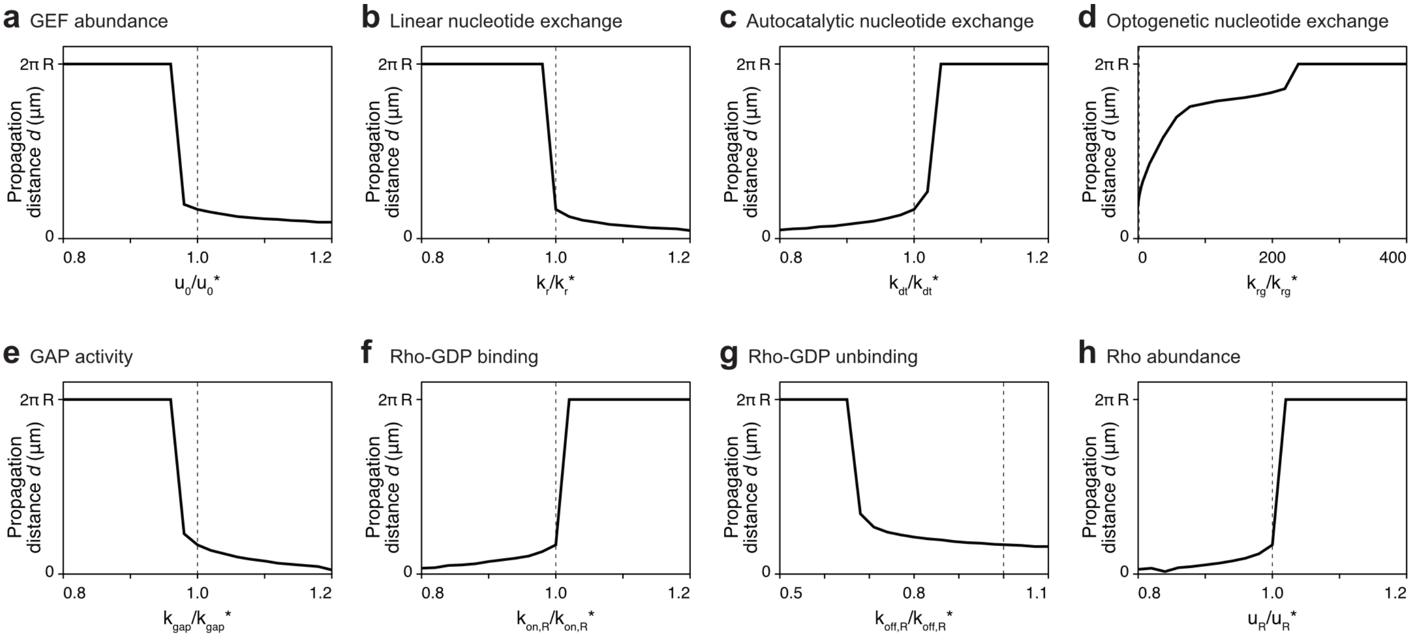


**Supplementary Fig. S6 | Transitions from localized Rho responses to propagating excitations as obtained by varying the relevant Rho model parameters in simulation.** The transitions are quantified in terms of the propagation distance of the excitation. The dashed vertical line indicates the default value for each of the model parameters. Note that the horizontal axis for the parameters $k_{\mathrm{rg}}$ (panel **d**) and $k_{\mathrm{off,R}}$ (panel **g**) differs from the other parameters.

Opto-GEF) has a passive ("in-dark") global effect on the cortical Rho activity by facilitating Rho excitations, compared to Opto-GEF where this effect is less pronounced. We were then inspired to explore a LARG-based optogenetic GEF (Opto-GEF*; Methods, Extended Data Fig. 7, Movie S5) to induce a stronger state perturbation compared to the Ect2-based Opto-GEF.

*Model implementation.* The full mechanism via which the autocatalytic Rho-GEF interaction is realized is not fully understood[7]. Similarly, the mechanism by which Opto-GEF* affects the endogenous Rho-GEF interactions without light activation has not been analysed beyond cell-level quantification of its effect on the cytoskeleton[34]. Consequently, it is not obvious which model parameter should represent the change from Opto-GEF to Opto-GEF*. Below, we discuss for each parameter of the Rho module whether varying this parameter could reproduce the observed difference between the two optogenetic constructs, and whether a plausible mechanism exists via which Opto-GEF* could mediate this parameter change. In Fig. S6, we show the wave propagation distance for all varied parameters to indicate the amount by which a parameter needs to be varied in order to transition from pinch responses to trigger waves.

**Abundance of additional GEFs $u_0$:** Increasing the abundance of additional GEFs cannot lead to a propagating excitation, since this reduces the amplitude of the Rho excitation and thus weakens state perturbations. We verified this reasoning by overexpression of constitutively active Ect2-T808A (Extended Data Fig. 6). However, reducing $u_0$ could in principle enable this transition (Fig. S6a). To achieve this, the Opto-GEF* construct would either need to reduce the GEF activity of the additional GEFs (since $u_0$ is an effective parameter, this would correspond to a lower value for $u_0$) or by downregulating the production of other GEFs. To our best knowledge, no mechanism exists that could realize these effects for LARG.

**Linear nucleotide exchange rate $k_{\mathrm{r}}$:** From a modeling perspective, a propagating excitation after localized illumination can be achieved by lowering the linear nucleotide exchange rate, whereas increasing this rate reduces the amplitude of excitations and does not support propagating waves (Fig. S6b). Heuristically, this is because a large linear rate means that at the non-equilibrium steady state of the system, a larger portion of Rho-GDP is converted into Rho-GTP and, therefore, the amount of Rho-GDP available in the event of an excitation is lower so that the peak Rho-GTP amplitude during an excitation is also lower. To cause a propagating excitation via this parameter, Opto-GEF* would need to attenuate the linear nucleotide exchange activity of the endogenous GEFs. Again, to our best knowledge, no such mechanism has been reported.

**Autocatalytic nucleotide exchange rate $k_{\mathrm{dt}}$:** Increasing the autocatalytic exchange rate can cause a transition from localized to propagating responses (Fig. S6c). Following a similar line of arguments as for $k_{\mathrm{r}}$, the amplitude of

the excitation is larger if the strength of this nonlinear term (which predominantly drives the excitation) is larger. For this parameter, we note that the specific nonlinear term in our model is only an effective representation of the necessary nonlinear interactions in the Rho system. As such, it is difficult to make statements about whether and how Opto-GEF* could interfere with the nonlinear interaction term, and we do not rule out this possibility.

**Optogenetic linear nucleotide exchange rate $k_{\mathrm{rg}}$:** Opto-GEF* is expected to have a stronger linear nucleotide exchange rate compared to Opto-GEF[35]. This effect cannot alter the Rho dynamics in a way such that stable propagating excitations are supported, most importantly because the optogenetic GEFs are not expected to have an effect outside the illuminated region. However, it can lead to a stronger localized excitation with stronger gradients, allowing the excitation to cover a larger distance across the oocyte membrane before decaying. In numerical simulations, we achieved waves that did not decay before colliding on the AP side when increasing the optogenetic linear nucleotide exchange rate by approximately a factor 300 compared to Opto-GEF (Fig. S6d). Based on previous studies[35], this effect is likely present to some degree in our system. However, it is not clear whether the effect in experiments is sufficiently strong to fully explain the observed transition to propagating excitations. In addition, this effect does not explain the elevated Rho response in non-illuminated cells[34], further indicating that this aspect is only partly responsible for the propagation.

**GAP rate $k_{\mathrm{gap}}$:** Similar to the autocatalytic exchange rate $k_{\mathrm{dt}}$, the GAP rate affects the strength of the excitation, where lower GAP rates lead to stronger excitations[2] (Fig. S6e). Consequently, wave propagation could be achieved if Opto-GEF* attenuated the GAP activity. To the best of our knowledge, there is, however, no known mechanism for how this effect would be realized in our system.

**Rho-GDP binding/unbinding rates $k_{\mathrm{on}}$ and $k_{\mathrm{off}}$:** Apart from affecting the nucleotide exchange, the Rho excitability can also be varied if the binding or unbinding rate of Rho from the cytosol to the membrane are affected[2]. A change in these rates (increase for $k_{\mathrm{on}}$, decrease for $k_{\mathrm{off}}$) essentially increases the amount of Rho-GDP on the membrane prior to excitation, which facilitates the propagation of the excitation into susceptible regions (Fig. S6f,g). To our best knowledge, no plausible mechanism exists that would explain how Opto-GEF* would decrease the Rho unbinding rate $k_{\mathrm{off}}$. For the binding process, however, one can conceive the following Opto-GEF*-assisted increase in Rho binding to the membrane: even without light activation, a fraction of Opto-GEF* may bind to the membrane through stochastic activation of the membrane anchor. These membrane-bound Opto-GEF* proteins may bind to cytosolic Rho-GDP via their DH domain[30] with higher specificity than the Ect2 counterparts[35], thereby assisting the membrane-binding of Rho-GDP.

**Total Rho concentration $u_{\mathrm{R}}$:** Finally, a similar result can be achieved if the total amount of Rho in the oocyte is increased[2], where the non-equilibrium steady states are shifted so that excitations are facilitated (Fig. S6h). To our best knowledge, however, no mechanism has been identified that would explain how Opto-GEF* affects the amount of Rho in the starfish oocyte.

Taken together, on the basis of the above theoretical analysis, we identify the binding process ($k_{\mathrm{on}}$), the difference in the linear activation rate of the optogenetic GEFs ($k_{\mathrm{rg}}$), as well as the nonlinear activation term, which in our model is accounted for in an effective manner ($k_{\mathrm{dt}}$) as the most likely candidates by which Opto-GEF* leads to propagating Rho excitations, possibly by a combination of multiple effects. Due to a lack of biomolecular analysis, we can, however, not rule out whether other mechanisms (i.e., processes represented by the other parameters discussed above) contribute to the wave propagation in the Opto-GEF* case. In simulations, we resolved to varying only one parameter (namely the autocatalytic activation rate $k_{\mathrm{dt}}$) for simplicity.

*Possible realization of the autocatalytic activation.* The term for the autocatalytic activation used in our model for the Rho dynamics has not been proven experimentally. One mechanism by which the proposed nonlinear interaction $u_{\mathrm{e0}} \cdot k_{\mathrm{dt}} \cdot u_{\mathrm{rt}}^2\, u_{\mathrm{rd}}$ might be realized on a molecular level is a two-step activation of a catalyzing protein that assists the nucleotide exchange. Such a mechanism has also been suggested for PLC$\epsilon$, a GEF for the small GTPase Ras and also an effector of Ras, based on structural analysis[36,37]. For the Rho system, such a two-step mechanism could, at least in principle, be realized by a protein that first needs to be recruited to the membrane by Rho-GTP from an abundant cytosolic pool ($u_{\mathrm{a1}}$) and is then converted into an active form ($u_{\mathrm{a2}}$) again by Rho-GTP where it then assists in the nucleotide exchange. A corresponding set of reaction terms would then read

$$f_{\mathrm{rt}}\big(u_{\mathrm{R}}|_{\mathcal{S}}, u_{\mathrm{rd}}, u_{\mathrm{rt}}, u_{\mathrm{a2}}\big) = u_{\mathrm{e0}} \cdot k_{\mathrm{r}}\, u_{\mathrm{rd}} + k_{\mathrm{dt,a}} \cdot u_{\mathrm{e0}} \cdot u_{\mathrm{a2}}\, u_{\mathrm{rd}} + u_{\mathrm{g}} \cdot k_{\mathrm{rg}}\, u_{\mathrm{rd}} - k_{\mathrm{gap}}\, u_{\mathrm{rt}}\,, \tag{44}$$

$$f_{\mathrm{a1}}\big(u_{\mathrm{rt}}, u_{\mathrm{a1}}\big) = k_{\mathrm{a1,on}}\, u_{\mathrm{rt}} - k_{\mathrm{a1,off}}\, u_{\mathrm{a1}}\,, \tag{45}$$

$$f_{\mathrm{a2}}\big(u_{\mathrm{rt}}, u_{\mathrm{a1}}, u_{\mathrm{a2}}\big) = k_{\mathrm{a2,on}}\, u_{\mathrm{a2,on}} \cdot u_{\mathrm{rt}} - k_{\mathrm{a2,off}}\, u_{\mathrm{a2}}\,, \tag{46}$$

where $f_{\rm rt}$ is the reaction term for the Rho-GTP protein species and $f_{\rm a1,a2}$ are the reaction terms for the intermediate complexes. The kinetic rates ($k_{\rm dt,a}$, $k_{\rm a1,on}$, $k_{\rm a2,on}$, $k_{\rm a1,off}$, and $k_{\rm a2,off}$) represent the formation/binding and unbinding of these intermediate complexes. For the sake of simplicity, we here assume that all GEFs including the Opto-GEF participate in the two-step activation. This can be generalized to a case where Opto-GEF does not participate in the feedback. In the limiting case where the reactions including the intermediate complexes are significantly faster than the Rho reactions, this specific set of equations in fact converges to the original set of equations (Eq. 31) with

$$k_{\rm dt} = \frac{k_{\rm dt,a}\, k_{\rm a1,on}\, k_{\rm a2,on}}{k_{\rm a1,off}\, k_{\rm a2,off}} \,.$$

As the reactions of the additional protein become slower, the autocatalytic effect is weakened and delayed, and the autocatalytic term in Eq. 31 becomes an approximation of the actual dynamics.

We emphasize that even though there is extensive evidence for the existence of some positive feedback[7], there is only little evidence for specific mechanisms, and the mechanism described above is purely speculative. For human Ect2, structural analysis indicates that at least the first part of the two-step interaction (binding of Ect2 to Rho with subsequent conformational change of Ect2, allowing for additional interactions with other Rho proteins) is possible[30], but these experimental results are insufficient to fully determine the mechanism underlying the nonlinear Rho activation. To unveil the real interactions, a biomolecular analysis of the autocatalysis is required.

## 5 Classification of contraction phenotypes

Upon exploring the light-induced contraction dynamics of starfish oocytes, we observe a variety of deformation phenotypes. Generically, the deformations can be classified by the spatial and temporal aspect of the contraction. Deformations can be (i) local and stationary ("pinches"), (ii) local and moving ("surface contraction waves"), (iii) global and stationary, or (iv) global and fluctuating. Out of these four classes we observe the former three, whereas globally fluctuating contractions (chaotic dynamics) have been previously reported for wild-type oocytes in the case of Ect2 overexpression[2,38]. In the following, we will relate the underlying biochemical dynamics to the observed phenotypes. For a graphical overview, see also Fig. 6.

Apart from a mere qualitative discussion of the phenotypes, we will also make a conceptual connection between the excitation threshold dynamics and the cell shape dynamics in the following. The observed deformation phenotypes are all induced by a specific spatio-temporal distribution of Rho-GTP on the oocyte membrane. More precisely, the Rho system needs to undergo an excursion in the (local) phase space, which produces a transient spike in Rho-GTP concentration. Such Rho-GTP excitability can be discussed in terms of a varying excitation threshold, as introduced in SI Section 3. High Rho-GTP concentrations lead to a local contraction of cytoskeletal actin and therefore causes shape deformations, which we quantify in terms of local membrane curvatures and Fourier shape decompositions (Methods). This allows us to relate the dynamics of the excitation threshold to the Fourier mode dynamics.

*Type I: local and stationary/"pinches".* Local and stationary deformations are characterized by domains that have negative curvature change after applying a light stimulus. Such pinches can be induced by localized illumination in oocytes that were injected with an optogenetic GEF variant. Upon illumination, the photosensitive domain conjugated with GEF acquires enhanced binding kinetics to the membrane anchor domain, significantly increasing the concentration of the optogenetic GEF proximal to membrane. This light-stimulus causes an excitation due to a threshold perturbation (Fig. 3a-c). For weak state perturbation susceptibility, this excitation is confined to the illuminated region or its immediate vicinity, so that contractions are only induced within the illuminated region. This leads to a local deformation that does not travel across the oocyte (Movie S6).

In terms of the Fourier mode dynamics, a pinch is characterized by a single excitation of all modes (single pinch) or of a subset of modes (multiple pinches with symmetry), as shown in Supplementary Fig. S7b. In particular, the specific subset of modes and the sign of the excitation is a strong signature of the symmetry of the light stimuli. For example, illumination at two opposite poles affects only even modes with $k{=}2,4,6,\dots$ (Movie S1); illumination at the corners of a virtual square affects even modes with $k{\geq}4$ (Movie S5).

*Type II: local and moving/"surface contraction waves".* Local and moving deformations are characterized by domains with negative curvature that travel across the cell. Such surface contraction waves can have various distinct driving mechanisms, which manifest themselves in different wave speeds.

First, SCWs can be guided by a native guiding cue, namely the Cdk1 gradient in wild-type oocytes[2,24]. In this case, the guiding cue marks a position on the membrane where the GEF concentration quickly increases. This corresponds to a threshold perturbation that is guided across the oocyte over time. The wave speed is determined by the speed of the guiding cue, i.e, by the slope and degradation rate of the Cdk1 gradient (Movie S7).

Second, SCWs can emerge from a global illumination combined with an internal guiding cue. In general, one would expect global illumination to cause homogeneous attachment of Opto-GEF to the membrane across the entire oocyte,

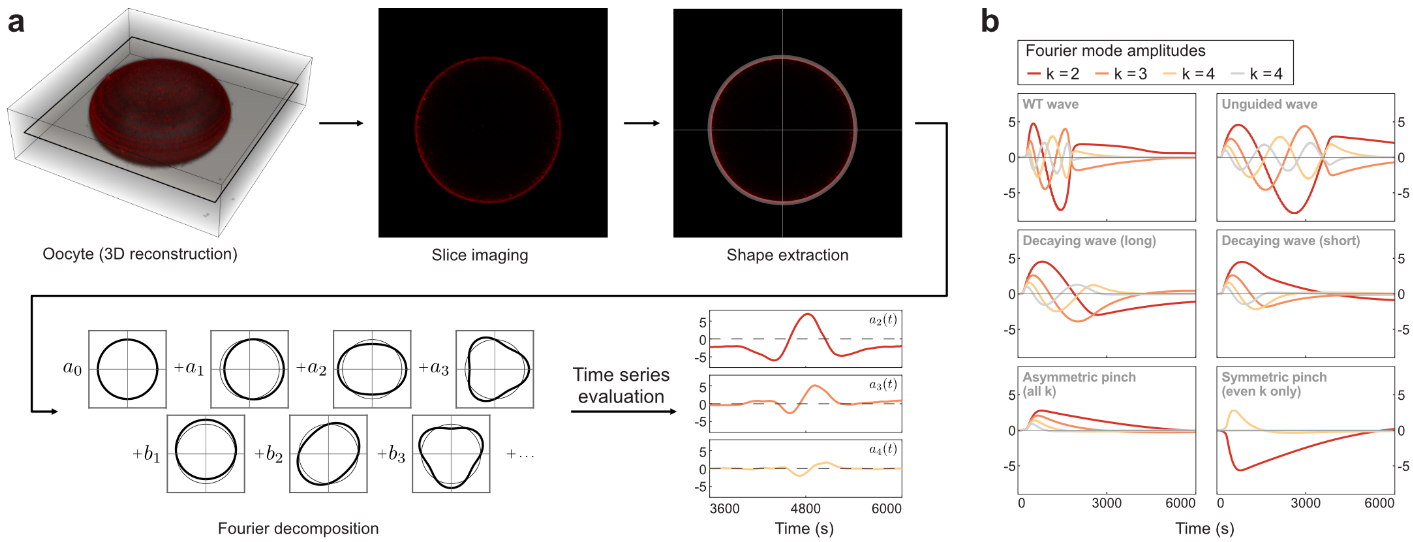


**Supplementary Fig. S7 | Extraction of oocyte shape from time series data. a,** Oocyte imaging and shape quantification pipeline. A horizontal slice of an oocyte stained by CellMask (Methods) was imaged and the outline of the oocyte in this slice was identified (top row). To quantify the shape, the outline was processed using a numerical Fourier transform in polar coordinates yielding amplitudes $a_k$ for cosine modes and $b_k$ for sine modes. The procedure was repeated for all snapshots to extract the time series of amplitudes (bottom row). **b,** Comparison of mode dynamics for different deformation phenotypes. Top row: surface contraction waves first compress, then stretch, then compress the oocyte along the propagation axis, yielding characteristic oscillations of the mode amplitudes $a_k(t)$, where the oscillation period depends on the wave speed $T \sim v^{-1}$. Center row: decaying waves initially have similar mode dynamcis as SCWs, but the oscillations are interrupted when the wave decays and the amplitudes relax back to their initial value. Bottom row: pinch deformations are characterized by a single mode amplitude peak and subsequent relaxation of all amplitudes. The symmetry of the deformation is reflected by the subset of modes that is activated and their sign. For example, only even modes are activated for symmetric deformations.

thus giving rise to a homogeneous contraction (see Type III). However, membrane binding of Opto-GEF requires the presence of the corresponding membrane anchors. As observed experimentally, the membrane anchors are not distributed homogeneously, but rather form a gradient along the AP-VP axis (Extended Data Fig. 6d-e, Movie S8). Along the AP-VP axis, the effective Opto-GEF binding therefore varies continuously, which means that the threshold perturbation is slowed down along this axis. This space-dependent delay is equivalent to a traveling wave; however, compared to wild-type SCWs, the wave propagates at a much higher velocity which is determined by the given anchor concentration gradient along the membrane, $\nabla u_\mathrm{a}|_\mathcal{S}$.

Third, SCWs can be realized without any guiding cue. For this, a threshold perturbation first needs to be triggered by a localized light stimulus, which then results in a Rho-GTP excitation in the illuminated region. As discussed in SI Section 3, this may develop into an unguided trigger wave propagating along the oocyte membrane. The speed of this wave is significantly slower than wild-type SCWs and, together with the propagation distance, is determined by the diffusion of Rho-GTP on the membrane, and by the characteristic time scale of the excitation dynamics. Altogether, the two extreme cases are captured by local pinches (weak state perturbation) and SCWs that travel across the entire oocyte (strong state perturbation) (Movie S6).

The Fourier mode dynamics for all these traveling waves differ significantly from the pinches (Supplementary Fig. S7b). In this case, the mode amplitudes $a_k(t)$ oscillate during the propagation of the SCW, where the oscillation frequency is roughly proportional to the mode number, $\omega_k \sim k$. The end of the SCW – for decaying waves as well as for complete SCWs – is characterised by a decay of all amplitudes. Note that the transitions from pinch to decaying wave and from decaying to complete wave are continuous.

*Type III: global and stationary.* For vanishingly shallow gradients of the anchor concentration, a global illumination of the oocyte causes a strong increase of the GEF concentration across the entire oocytes' perimeter, with no or negligible delay. Thus, the system will almost synchronously undergo an excursion in phase space, resulting in peaked Rho activity along the entire surface. This is, in essence, a limit case of type II deformations after global illumination with $\nabla u_\mathrm{a}|_\mathcal{S} \to 0$. The resulting actomyosin activity is approximately homogeneous across the oocyte's cortex, leading to a global compression of the oocyte. This global compression is counteracted by internal constraints, in particular cytoplasmic pressure resulting from volume conservation, which tends to cause cortex rupture and disintegration of cellular material (Movie S11).

*Type IV: global and fluctuating.* Following the above classification scheme, a fourth category of oocyte deformations can be

defined, where Rho-GTP activity is elevated across the entire oocyte at the same time but without synchronization. Such deformations would be caused by oscillatory Rho dynamics (i.e., a limit cycle in the Rho phase space), and have been reported previously for Ect2 overexpression in wild-type oocytes[2,38,39] and at the cytokinetic furrow during cell division[8]. For the optogenetic setup, these dynamics were not observed, as they were likely overlayed by dynamics of type III.

## Movie captions

**S1 Reversible oocyte deformations driven by patterned illumination with Opto-GEF assay.** | Representative video of a prophase-arrested starfish oocyte undergoing reversible shape changes driven by patterned illumination. Oocyte expresses Opto-GEF assay and was continuously activated with two illumination sites (488 nm) at 1 Hz for 1hr before the illumination is turned off. Scale bar: 50 $\mu$m.

**S2 Mid-plane view of membrane Rho-GTP dynamics driven by continuous global illumination.** | Representative video of a prophase-arrested starfish oocyte showing oscillatory Rho dynamics under continuous global activation. Oocyte expresses Opto-GEF assay and the active Rho sensor and was placed under global illumination (488 nm) at 0.1 Hz for 30min. Scale bar: 50 $\mu$m.

**S3 Near-membrane view of membrane Rho-GTP dynamics driven by continuous global illumination.** | Representative video of a prophase-arrested starfish oocyte showing oscillatory Rho dynamics under continuous global activation. Oocyte expresses Opto-GEF assay and the active Rho sensor and was placed under global illumination (488 nm) at 0.1 Hz for 30min. The imaging was focused on the bottom plane in chamber to capture Rho dynamics near membrane. Video was made from the maximal intensity projection from 3 consecutive z-planes that are each 1 $\mu$m apart. Scale bar: 50 $\mu$m.

**S4 Simulation of a self-sustained traveling Rho wave following local activation.** | Regional illumination (cyan box) locally lowers the excitation threshold and induces a localized Rho excitation. The resulting heterogeneous Rho-GTP concentration profile causes strong diffusive fluxes and thus triggers an excitation due to lateral activation in the around the illuminated region. This excitation travels along the circumference of the oocyte until the two peaks collide and annihilate.

**S5 Reversible oocyte deformations driven by patterned illumination expressing Opto-GEF* assay.** | Oocyte expresses Opto-GEF* assay and was continuously activated with four illumination sites (488 nm) at 0.1 Hz for 20 min and then removed. Cyan boxes show the outline of illumination sites. Scale bar: 50 $\mu$m.

**S6 Opto-GEF* assay-expressing oocytes exhibit pinching or unguided SCW upon local activation.** | Two representative oocytes expressing Opto-GEF* assay was placed under local activation at 1 Hz for 3 min before illumination was removed. With varied protein expression level and activation site area, the oocytes were observed to show localized pinching deformation (left) or a propagating unguided surface contraction wave (SCW, right) respectively. Cyan boxes show the outline of illumination sites and the ring overlay visualizes the change of cell surface curvatures. Scale bar: 50 $\mu$m.

**S7 Wild-type oocyte exhibits guided SCW under hormone induction.** | A representative wild-type oocyte performing guided surface contraction wave (SCW) after hormone (1MA) induction of meiosis. The oocyte expresses active Rho sensor that was traced in time-lapse imaging. The ring overlay visualizes the change of cell surface curvatures. Scale bar: 50 $\mu$m.

**S8 Opto-GEF assay-expressing oocyte exhibits guided SCW under continued global activation.** | A representative Opto-GEF assay-expressing oocyte placed under continued global activation at 0.1 Hz. The oocytes were observed to display variable time till the pole-to-pole membrane recruitment asymmetry was configured and a guided surface contraction wave (SCW) follows. Cyan boxes show the outline of illumination sites and the ring overlay visualizes the change of cell surface curvatures. Scale bar: 50 $\mu$m.

**S9 Irreversible Opto-GEF assay-expressing oocyte lysis driven by global illumination.** | Representative videos of prophase-arrested starfish oocytes undergoing irreversible cell lysis driven by global illumination at long time. Oocyte expresses Opto-GEF assay and was continuously activated at 0.1 Hz on the nucleus plane. The oocytes that performed guided surface contraction waves (SCWs) were observed to undergo irreversible lysis unanimously after the SCW. Scale bar: 50 $\mu$m.

**S10 Irreversible Opto-GEF* assay-expressing oocyte lysis driven by global illumination.** | Representative videos of prophase-arrested starfish oocytes undergoing irreversible cell lysis driven by global illumination. Oocyte expresses Opto-GEF* assay and was continuously activated at 0.1 Hz on the nucleus plane. Scale bar: 50 $\mu$m.

**S11 Extreme irreversible Opto-GEF assay-expressing oocyte lysis driven by global illumination.** | Representative videos of prophase-arrested starfish oocytes undergoing irreversible cell lysis driven by global illumination. Oocyte expresses Opto-GEF assay and was continuously activated at 0.1 Hz on the nucleus plane. Scale bar: 50 $\mu$m.

## References


[1] Lukasz J. Bugaj, Atri T. Choksi, Colin K. Mesuda, Ravi S. Kane, and David V. Schaffer. Optogenetic protein clustering and signaling activation in mammalian cells. *Nature Methods*, 10(3):249–252, 2013.

[2] Manon C. Wigbers, Tzer Han Tan, Fridtjof Brauns, Jinghui Liu, S. Zachary Swartz, Erwin Frey, and Nikta Fakhri. A hierarchy of protein patterns robustly decodes cell shape information. *Nature Physics*, 17(5):578–584, 2021.

[3] J. Tailleur, G. Gompper, M.C. Marchetti, J.M. Yeomans, and C. Salomon. *Active Matter and Nonequilibrium Statistical Physics: Lecture Notes of the Les Houches Summer School: Volume 112, September 2018*. Lecture Notes of the Les Houches Summer School. OUP Oxford, 2022.

[4] Angika Basant and Michael Glotzer. Spatiotemporal Regulation of RhoA during Cytokinesis. *Current Biology*, 28(9):R570–R580, 2018.

[5] Latasha P. Wright and Mark R. Philips. Thematic review series: Lipid Posttranslational Modifications CAAX modification and membrane targeting of Ras. *Journal of Lipid Research*, 47(5):883–891, 2006.

[6] Geoffrey Grimmett and David Stirzaker. *Probability and random processes*. Oxford University Press, 2020.

[7] William M. Bement, Andrew B. Goryachev, Ann L. Miller, and George von Dassow. Patterning of the cell cortex by Rho GTPases. *Nature Reviews Molecular Cell Biology*, pages 1–19, 2024.

[8] William M. Bement, Marcin Leda, Alison M. Moe, Angela M. Kita, Matthew E. Larson, Adriana E. Golding, Courtney Pfeuti, Kuan-Chung Su, Ann L. Miller, Andrew B. Goryachev, and George von Dassow. Activator–inhibitor coupling between Rho signalling and actin assembly makes the cell cortex an excitable medium. *Nature Cell Biology*, 17(11):1471–1483, 2015.

[9] Ani Michaud, Marcin Leda, Zachary T. Swider, Songeun Kim, Jiaye He, Jennifer Landino, Jenna R. Valley, Jan Huisken, Andrew B. Goryachev, George von Dassow, and William M. Bement. A versatile cortical pattern-forming circuit based on Rho, F-actin, Ect2, and RGA-3/4. *Journal of Cell Biology*, 221(8):e202203017, 2022.

[10] Andrew B. Goryachev and Marcin Leda. Many roads to symmetry breaking: molecular mechanisms and theoretical models of yeast cell polarity. *Molecular Biology of the Cell*, 28(3):370–380, 2017.

[11] Nils Klughammer, Johanna Bischof, Nikolas D. Schnellbächer, Andrea Callegari, Péter Lénárt, and Ulrich S. Schwarz. Cytoplasmic flows in starfish oocytes are fully determined by cortical contractions. *PLoS computational biology*, 14(11):e1006588, 2018.

[12] Rukshala Illukkumbura, Tom Bland, and Nathan W. Goehring. Patterning and polarization of cells by intracellular flows. *Current Opinion in Cell Biology*, 62:123–134, 2020.

[13] Mirjam Mayer, Martin Depken, Justin S. Bois, Frank Jülicher, and Stephan W. Grill. Anisotropies in cortical tension reveal the physical basis of polarizing cortical flows. *Nature*, 467(7315):617–621, 2010.

[14] Justin S. Bois, Frank Jülicher, and Stephan W. Grill. Pattern Formation in Active Fluids. *Physical Review Letters*, 106(2):028103, 2011.

[15] Masatoshi Nishikawa, Sundar Ram Naganathan, Frank Jülicher, and Stephan W. Grill. Controlling contractile instabilities in the actomyosin cortex. *eLife*, 6:e19595, 2017.

[16] Peter J. Foster, Sebastian Fürthauer, and Nikta Fakhri. Active mechanics of sea star oocytes. *bioRxiv*, page 2022.04.22.489189, 2022.

[17] Shuh Narumiya, Masahiro Tanji, and Toshimasa Ishizaki. Rho signaling, ROCK and mDia1, in transformation, metastasis and invasion. *Cancer and Metastasis Reviews*, 28(1-2):65–76, 2009.

[18] Sifan Yin, Bo Li, and Xi-Qiao Feng. Bio-chemo-mechanical theory of active shells. *Journal of the Mechanics and Physics of Solids*, 152:104419, 2021.

[19] John Ross, Stefan C. Müller, and Christian Vidal. Chemical Waves. *Science*, 240(4851):460–465, 1988.

[20] Ehud Meron. Pattern formation in excitable media. *Physics Reports*, 218(1):1–66, 1992.

[21] Rashmi C. Desai and Raymond Kapral. *Dynamics of Self-Organized and Self-Assembled Structures*. Cambridge University Press, 3 2009.

[22] Jeremy B. Chang and James E. Ferrell Jr. Mitotic trigger waves and the spatial coordination of the Xenopus cell cycle. *Nature*, 500(7464):603–607, 2013.

[23] Lendert Gelens, Graham A. Anderson, and James E. Ferrell. Spatial trigger waves: positive feedback gets you a long way. *Molecular Biology of the Cell*, 25(22):3486–3493, 2014.

[24] Johanna Bischof, Christoph A. Brand, Kálmán Somogyi, Imre Májer, Sarah Thome, Masashi Mori, Ulrich S. Schwarz, and Péter Lénárt. A cdk1 gradient guides surface contraction waves in oocytes. *Nature Communications*, 8(1):849, 2017.

[25] Hélène A. Benink and William M. Bement. Concentric zones of active RhoA and Cdc42 around single cell wounds. *The Journal of Cell Biology*, 168(3):429–439, 2005.

[26] Johanna Bischof. *The molecular mechanism of surface contraction waves in the starfish oocyte*. PhD thesis, 7 2016.

[27] Takeshi Sakamoto, John Limouze, Christian A. Combs, Aaron F. Straight, and James R. Sellers. Blebbistatin, a Myosin II Inhibitor, Is Photoinactivated by Blue Light. *Biochemistry*, 44(2):584–588, 2005.

[28] Jonathan Stricker, Yvonne Aratyn-Schaus, Patrick W. Oakes, and Margaret L. Gardel. Spatiotemporal Constraints on the Force-Dependent Growth of Focal Adhesions. *Biophysical Journal*, 100(12):2883–2893, 2011.

[29] Ian Linsmeier, Shiladitya Banerjee, Patrick W. Oakes, Wonyeong Jung, Taeyoon Kim, and Michael P. Murrell. Disordered actomyosin networks are sufficient to produce cooperative and telescopic contractility. *Nature Communications*, 7(1):12615, 2016.

[30] Mengran Chen, Han Pan, Lingfei Sun, Peng Shi, Yikan Zhang, Le Li, Yuxing Huang, Jianhui Chen, Peng Jiang, Xianyang Fang, Congying Wu, and Zhucheng Chen. Structure and regulation of human epithelial cell transforming 2 protein. *Proceedings of the National Academy of Sciences*, 117(2):1027–1035, 2020.

[31] Amir Taslimi, Brian Zoltowski, Jose G. Miranda, Gopal Pathak, Robert M. Hughes, and Chandra L. Tucker. Optimized second generation CRY2/CIB dimerizers and photoactivatable Cre recombinase. *Nature chemical biology*, 12(6):425–430, 2016.

[32] Mamta Jaiswal, Lothar Gremer, Radovan Dvorsky, Lars Christian Haeusler, Ion C. Cirstea, Katharina Uhlenbrock, and Mohammad Reza Ahmadian. Mechanistic Insights into Specificity, Activity, and Regulatory Elements of the Regulator of G-protein Signaling (RGS)-containing Rho-specific Guanine Nucleotide Exchange Factors (GEFs) p115, PDZ-RhoGEF (PRG), and Leukemia-associated RhoGEF (LARG)*. *Journal of Biological Chemistry*, 286(20):18202–18212, 2011.

[33] Elizabeth Wagner and Michael Glotzer. Local RhoA activation induces cytokinetic furrows independent of spindle position and cell cycle stage. *Journal of Cell Biology*, 213(6):641–649, 2016.

[34] Elizabeth Wagner. *Optogenetic analysis of RhoA-mediated furrow formation during cytokinesis*. PhD thesis, 8 2016.

[35] Romana Kristelly, Guang Gao, and John J.G. Tesmer. Structural Determinants of RhoA Binding and Nucleotide Exchange in Leukemia-associated Rho Guanine-Nucleotide Exchange Factor*. *Journal of Biological Chemistry*, 279(45):47352–47362, 2004.

[36] Sue Goo Rhee. Regulation of Phosphoinositide-Specific Phospholipase C*. *Annual Review of Biochemistry*, 70(1):281–312, 2001.

[37] Tom D. Bunney, Richard Harris, Natalia Lamuño Gandarillas, Michelle B. Josephs, S. Mark Roe, S. Caroline Sorli, Hugh F. Paterson, Fernando Rodrigues-Lima, Diego Esposito, Chris P. Ponting, Peter Gierschik, Laurence H. Pearl, Paul C. Driscoll, and Matilda Katan. Structural and Mechanistic Insights into Ras Association Domains of Phospholipase C Epsilon. *Molecular Cell*, 21(4):495–507, 2006.

[38] Tzer Han Tan, Jinghui Liu, Pearson W. Miller, Melis Tekant, Jörn Dunkel, and Nikta Fakhri. Topological turbulence in the membrane of a living cell. *Nature Physics*, 16(6):657–662, 2020.

[39] Jinghui Liu, Jan F. Totz, Pearson W. Miller, Alasdair D. Hastewell, Yu-Chen Chao, Jörn Dunkel, and Nikta Fakhri. Topological braiding and virtual particles on the cell membrane. *Proceedings of the National Academy of Sciences*, 118(34):e2104191118, 2021.
